# Supplementary material for: Erratum to: Almost complex structures in 6D with non-degenerate Nijenhuis tensors and large symmetry groups
Source: arXiv:1612.09493 ancillary file (2016-12-18)
Supplement: Supplementary file 1 [file Maple_BKHW_for_erratum.pdf]

```
> restart:with(DifferentialGeometry): with(Tensor): with(Tools): with(LieAlgebras):
```

```
h > dimM:=6;
```

*dimM := 6*

(1)

```
g > cohom_algfromten:=proc(baseten,isotropyten)
  local i, j, basebase, vertbase, vertvert, StrBaseArray, StrVertArray, StrActionArray,
  StrIsoArray, GetBaseStrConstsVector, GetVertStrConstsVector, GetActionStrConstsVector,
  GetIsoStrConstsVector, FrameName, FrameDim, VertDim, mDim, conbas, tenframe, tLieBracket,
  tVertBracket, tHAction, tEndBracket;

  FrameName:=DGinfo(baseten,"ObjectFrame");
  conbas:=DGinfo(FrameName,"FrameBaseVectors");
  tenframe:=map(x->convert(x,DGtensor),conbas);
  FrameDim:=DGinfo(FrameName,"FrameBaseDimension");
  VertDim:=nops(isotropyten);
  mDim:=FrameDim-VertDim;

  tLieBracket:=(x,y)->ContractIndices(evalDG(x &t y),baseten,[[1,1],[2,2]]);
  GetBaseStrConstsVector:=(x,y)->GetComponents(tLieBracket(x,y), tenframe);
  tHAction:=(x,y)->ContractIndices(x,y,[[2,1]]);
  GetActionStrConstsVector:=(x,y)->GetComponents(tHAction(x,y), tenframe);
  tEndBracket:=(x,y)->evalDG(ContractIndices(x,y,[[2,1]]) &minus ContractIndices(y,x,[[2,1]]));
  GetIsoStrConstsVector:=(x,y)->GetComponents(tEndBracket(x,y), isotropyten);

  for i from 1 to mDim do for j from i+1 to mDim do StrBaseArray[VertDim+i,VertDim+j]:=
  GetBaseStrConstsVector(tenframe[VertDim+i],tenframe[VertDim+j]); end do end do;
  for i from 1 to VertDim do for j from 1 to mDim do StrActionArray[i,VertDim+j]:=
  GetActionStrConstsVector(isotropyten[i],tenframe[VertDim+j]); end do end do;
  for i from 1 to VertDim do for j from i+1 to VertDim do StrIsoArray[i,j]:=
  GetIsoStrConstsVector(isotropyten[i],isotropyten[j]); end do end do;

  basebase:= seq(seq([o||i,o||j]=add(StrBaseArray[VertDim+i,VertDim+j][VertDim+k]*o||k,k=1..
  mDim)+add(StrBaseArray[VertDim+i,VertDim+j][k]*r||k,k=1..VertDim),j=1+i..mDim),i=1..mDim);
  vertbase:=seq(seq([r||i,o||j]=add(StrActionArray[i,VertDim+j][VertDim+k]*o||k,k=1..mDim)+add
  (StrActionArray[i,VertDim+j][k]*r||k,k=1..VertDim),j=1..mDim),i=1..VertDim);
  vertvert:=seq(seq([r||i,r||j]=add(StrIsoArray[i,j][k]*r||k,k=1..VertDim),j=1+i..VertDim),i=1.
  .VertDim);
```

```
return [basebase,vertbase,vertvert],[seq(r||i,i=1..VertDim),seq(o||i,i=1..mDim)];
```

```
end proc;
```

This function takes two tensors describing the brackets and isotropy of a Lie algebra and converts it to structure equations.

Section 1: h=r

```
V > MrepMat := [Matrix(10, 10, {(1, 1) = 0, (1, 2) = 0, (1, 3) = 0, (1, 4) = 0, (1, 5) = 0, (1, 6) = 0, (1, 7) = 0, (1, 8) = 0, (1, 9) = 0, (1, 10) = 0, (2, 1) = 0, (2, 2) = -1, (2, 3) = 0, (2, 4) = 0, (2, 5) = 0, (2, 6) = 0, (2, 7) = 0, (2, 8) = 0, (2, 9) = 0, (2, 10) = 0, (3, 1) = 0, (3, 2) = 0, (3, 3) = -1, (3, 4) = 0, (3, 5) = 0, (3, 6) = 0, (3, 7) = 0, (3, 8) = 0, (3, 9) = 0, (3, 10) = 0, (4, 1) = 0, (4, 2) = 0, (4, 3) = 0, (4, 4) = -2, (4, 5) = 0, (4, 6) = 0, (4, 7) = 0, (4, 8) = 0, (4, 9) = 0, (4, 10) = 0, (5, 1) = 0, (5, 2) = 0, (5, 3) = 0, (5, 4) = 0, (5, 5) = 1, (5, 6) = 0, (5, 7) = 0, (5, 8) = 0, (5, 9) = 0, (5, 10) = 0, (6, 1) = 0, (6, 2) = 0, (6, 3) = 0, (6, 4) = 0, (6, 5) = 0, (6, 6) = 1, (6, 7) = 0, (6, 8) = 0, (6, 9) = 0, (6, 10) = 0, (7, 1) = 0, (7, 2) = 0, (7, 3) = 0, (7, 4) = 0, (7, 5) = 0, (7, 6) = 0, (7, 7) = -1, (7, 8) = 0, (7, 9) = 0, (7, 10) = 0, (8, 1) = 0, (8, 2) = 0, (8, 3) = 0, (8, 4) = 0, (8, 5) = 0, (8, 6) = 0, (8, 7) = 0, (8, 8) = -1, (8, 9) = 0, (8, 10) = 0, (9, 1) = 0, (9, 2) = 0, (9, 3) = 0, (9, 4) = 0, (9, 5) = 0, (9, 6) = 0, (9, 7) = 0, (9, 8) = 0, (9, 9) = 0, (9, 10) = 0, (10, 1) = 0, (10, 2) = 0, (10, 3) = 0, (10, 4) = 0, (10, 5) = 0, (10, 6) = 0, (10, 7) = 0, (10, 8) = 0, (10, 9) = 0, (10, 10) = 0}), Matrix(10, 10, {(1, 1) = 0, (1, 2) = 0, (1, 3) = 0, (1, 4) = 0, (1, 5) = (60/803)*u1+(4/2409)*u2+(8627/2409)*u5, (1, 6) = -(18/13)*u3+(823/104)*u4-5*u6, (1, 7) = 0, (1, 8) = 0, (1, 9) = 0, (1, 10) = 0, (2, 1) = 1, (2, 2) = 0, (2, 3) = 0, (2, 4) = 0, (2, 5) = 0, (2, 6) = 0, (2, 7) = 0, (2, 8) = 0, (2, 9) = (597/1606)*u1+(1967/4818)*u2-(2671/2409)*u5, (2, 10) = (7/39)*u3-(2005/312)*u4+6*u6, (3, 1) = 0, (3, 2) = 0, (3, 3) = 0, (3, 4) = 0, (3, 5) = 0, (3, 6) = 0, (3, 7) = 0, (3, 8) = 0, (3, 9) = (109/117)*u3-(2461/936)*u4+(5/3)*u6, (3, 10) = u2, (4, 1) = 0, (4, 2) = 0, (4, 3) = 1, (4, 4) = 0, (4, 5) = 0, (4, 6) = 0, (4, 7) = (46/117)*u3-(2317/936)*u4+(5/3)*u6, (4, 8) = u5, (4, 9) = 0, (4, 10) = 0, (5, 1) = 0, (5, 2) = 0, (5, 3) = 0, (5, 4) = 0, (5, 5) = 0, (5, 6) = 0, (5, 7) = 0, (5, 8) = 0, (5, 9) = 0, (5, 10) = 0, (6, 1) = 0, (6, 2) = 0, (6, 3) = 0, (6, 4) = 0, (6, 5) = 0, (6, 6) = 0, (6, 7) = 0, (6, 8) = 0, (6, 9) = 0, (6, 10) = 0, (7, 1) = 0, (7, 2) = 0, (7, 3) = 0, (7, 4) = 0, (7, 5) = 0, (7, 6) = 0, (7, 7) = 0, (7, 8) = 0, (7, 9) = 1, (7, 10) = 0, (8, 1) = 0, (8, 2) = 0, (8, 3) = 0, (8, 4) = 0, (8, 5) = 0, (8, 6) = 0, (8, 7) = 0, (8, 8) = 0, (8, 9) = 0, (8, 10) = 1, (9, 1) = 0, (9, 2) = 0, (9, 3) = 0, (9, 4) = 0, (9, 5) = -1, (9, 6) = 0, (9, 7) = 0, (9, 8) = 0, (9, 9) = 0, (9, 10) = 0, (10, 1) = 0, (10, 2) = 0, (10, 3) = 0, (10, 4) = 0, (10, 5) = 0, (10, 6) = -1, (10, 7) = 0, (10, 8) = 0, (10, 9) = 0, (10, 10) = 0}), Matrix(10, 10, {(1, 1) = 0, (1, 2) = 0, (1, 3) = 0, (1, 4) = 0, (1, 5) = -(8/117)*u3+(136/117)*u4+(1/3)*u6, (1, 6) = -(1357/4818)*u1+(5573/4818)*u2-(7597/2409)*u5, (1, 7) = 0,
```

```
(1, 8) = 0, (1, 9) = 0, (1, 10) = 0, (2, 1) = 0, (2, 2) = 0, (2, 3) = 0, (2, 4) = 0, (2, 5) =
0, (2, 6) = 0, (2, 7) = 0, (2, 8) = 0, (2, 9) = -(1/3)*u3+(307/24)*u4-13*u6, (2, 10) = u1,
(3, 1) = 1, (3, 2) = 0, (3, 3) = 0, (3, 4) = 0, (3, 5) = 0, (3, 6) = 0, (3, 7) = 0, (3, 8) =
0, (3, 9) = (40/803)*u1-(5083/2409)*u2+(6019/2409)*u5, (3, 10) = u3, (4, 1) = 0, (4, 2) = -1,
(4, 3) = 0, (4, 4) = 0, (4, 5) = 0, (4, 6) = 0, (4, 7) = (397/1606)*u1-(3935/4818)*u2+
(5167/2409)*u5, (4, 8) = u6, (4, 9) = 0, (4, 10) = 0, (5, 1) = 0, (5, 2) = 0, (5, 3) = 0, (5,
4) = 0, (5, 5) = 0, (5, 6) = 0, (5, 7) = 0, (5, 8) = 0, (5, 9) = 0, (5, 10) = 0, (6, 1) = 0,
(6, 2) = 0, (6, 3) = 0, (6, 4) = 0, (6, 5) = 0, (6, 6) = 0, (6, 7) = 0, (6, 8) = 0, (6, 9) =
0, (6, 10) = 0, (7, 1) = 0, (7, 2) = 0, (7, 3) = 0, (7, 4) = 0, (7, 5) = 0, (7, 6) = 0, (7,
7) = 0, (7, 8) = 0, (7, 9) = 0, (7, 10) = -3, (8, 1) = 0, (8, 2) = 0, (8, 3) = 0, (8, 4) = 0,
(8, 5) = 0, (8, 6) = 0, (8, 7) = 0, (8, 8) = 0, (8, 9) = 3, (8, 10) = 0, (9, 1) = 0, (9, 2) =
0, (9, 3) = 0, (9, 4) = 0, (9, 5) = 0, (9, 6) = -3, (9, 7) = 0, (9, 8) = 0, (9, 9) = 0, (9,
10) = 0, (10, 1) = 0, (10, 2) = 0, (10, 3) = 0, (10, 4) = 0, (10, 5) = 3, (10, 6) = 0, (10,
7) = 0, (10, 8) = 0, (10, 9) = 0, (10, 10) = 0}}, Matrix(10, 10, {(1, 1) = 0, (1, 2) = 0, (1,
3) = 0, (1, 4) = 0, (1, 5) = 0, (1, 6) = 0, (1, 7) = 0, (1, 8) = 0, (1, 9) = 0, (1, 10) = 0,
(2, 1) = 0, (2, 2) = 0, (2, 3) = 0, (2, 4) = 0, (2, 5) = (16/117)*u3-(623/117)*u4+(16/3)*u6,
(2, 6) = -(956/2409)*u1-(164/2409)*u2+(416/2409)*u5, (2, 7) = 0, (2, 8) = 0, (2, 9) = 0, (2,
10) = 0, (3, 1) = 0, (3, 2) = 0, (3, 3) = 0, (3, 4) = 0, (3, 5) = -(20/803)*u1+(2140/2409)*u2
-(2608/2409)*u5, (3, 6) = -(16/39)*u3-(1/39)*u4, (3, 7) = 0, (3, 8) = 0, (3, 9) = 0, (3, 10)
= 0, (4, 1) = 2, (4, 2) = 0, (4, 3) = 0, (4, 4) = 0, (4, 5) = 0, (4, 6) = 0, (4, 7) = 0, (4,
8) = 0, (4, 9) = (140/803)*u1-(2132/2409)*u2+(5408/2409)*u5, (4, 10) = u4, (5, 1) = 0, (5, 2)
= 0, (5, 3) = 0, (5, 4) = 0, (5, 5) = 0, (5, 6) = 0, (5, 7) = 0, (5, 8) = 0, (5, 9) = 0, (5,
10) = 0, (6, 1) = 0, (6, 2) = 0, (6, 3) = 0, (6, 4) = 0, (6, 5) = 0, (6, 6) = 0, (6, 7) = 0,
(6, 8) = 0, (6, 9) = 0, (6, 10) = 0, (7, 1) = 0, (7, 2) = 0, (7, 3) = 0, (7, 4) = 0, (7, 5) =
0, (7, 6) = -6, (7, 7) = 0, (7, 8) = 0, (7, 9) = 0, (7, 10) = 0, (8, 1) = 0, (8, 2) = 0, (8,
3) = 0, (8, 4) = 0, (8, 5) = 6, (8, 6) = 0, (8, 7) = 0, (8, 8) = 0, (8, 9) = 0, (8, 10) = 0,
(9, 1) = 0, (9, 2) = 0, (9, 3) = 0, (9, 4) = 0, (9, 5) = 0, (9, 6) = 0, (9, 7) = 0, (9, 8) =
0, (9, 9) = 0, (9, 10) = 0, (10, 1) = 0, (10, 2) = 0, (10, 3) = 0, (10, 4) = 0, (10, 5) = 0,
(10, 6) = 0, (10, 7) = 0, (10, 8) = 0, (10, 9) = 0, (10, 10) = 0}}]:
```

In these matrices, the variables  $u_1..u_6$  parametrize the cohomology classes  $[\phi]$  of indecomposable modules.

```
V80 > HData:=LieAlgebraData(MrepMat,h):DGsetup(HData);
```

*Lie algebra: h*

(2)

```
V > DGsetup([seq(v||i,i=1..dimM)],m);
```

*frame name: m*

(3)

```
m > DGsetup([seq(w||i,i=1..10)],g);
```

*frame name: g*

(4)

```
g > grep:=Representation(h,g,MrepMat):
```

```
G > ChangeFrame(g);
```

15

$g$

(5)

```
g > L2M:=GenerateForms(DGinfo(g,"FrameBaseForms")[5..10],2);
```

```
L2M:=[dw5 ∧ dw6, dw5 ∧ dw7, dw5 ∧ dw8, dw5 ∧ dw9, dw5 ∧ dw10, dw6 ∧ dw7, dw6 ∧ dw8, dw6 ∧ dw9, dw6 ∧ dw10, dw7 ∧ dw8,  
dw7 ∧ dw9, dw7 ∧ dw10, dw8 ∧ dw9, dw8 ∧ dw10, dw9 ∧ dw10]
```

(6)

```
g > brakspace:=GenerateTensors([L2M,DGinfo(g,"FrameBaseVectors")]):
```

```
g > genbrak:=evalDG(add(a||i*brakspace[i],i=1..nops(brakspace))):
```

```
g > gisoten:=map(x->convert(x,DGtensor,[["con_bas", "cov_bas"], []]),MrepMat);
```

$$\begin{aligned} gisoten := & \left[ - (D_{w2} dw2) - (D_{w3} dw3) - ((2 D_{w4} dw4) + D_{w5} dw5 + D_{w6} dw6 - (D_{w7} dw7) - (D_{w8} dw8), \left( \left( \frac{60 u1}{803} \right. \right. \right. \\ & + \frac{4 u2}{2409} + \frac{8627 u5}{2409} \Big) D_{w1} \Big) dw5 - \left( \left( \left( \frac{18 u3}{13} - \frac{823 u4}{104} + 5 u6 \right) D_{w1} \right) dw6 \right) + D_{w2} dw1 + \left( \left( \frac{597 u1}{1606} + \frac{1967 u2}{4818} \right. \right. \\ & - \frac{2671 u5}{2409} \Big) D_{w2} \Big) dw9 + \left( \left( \frac{7 u3}{39} - \frac{2005 u4}{312} + 6 u6 \right) D_{w2} \right) dw10 + \left( \left( \frac{109 u3}{117} - \frac{2461 u4}{936} + \frac{5 u6}{3} \right) D_{w3} \right) dw9 \\ & + (u2 D_{w3}) dw10 + D_{w4} dw3 + \left( \left( \frac{46 u3}{117} - \frac{2317 u4}{936} + \frac{5 u6}{3} \right) D_{w4} \right) dw7 + (u5 D_{w4}) dw8 + D_{w7} dw9 + D_{w8} dw10 \\ & - (D_{w9} dw5) - (D_{w10} dw6), - \left( \left( \left( \frac{8 u3}{117} - \frac{136 u4}{117} - \frac{u6}{3} \right) D_{w1} \right) dw5 \right) - \left( \left( \left( \frac{1357 u1}{4818} - \frac{5573 u2}{4818} \right. \right. \right. \\ & + \frac{7597 u5}{2409} \Big) D_{w1} \Big) dw6 \Big) - \left( \left( \left( \frac{u3}{3} - \frac{307 u4}{24} + 13 u6 \right) D_{w2} \right) dw9 \right) + (u1 D_{w2}) dw10 + D_{w3} dw1 + \left( \left( \frac{40 u1}{803} - \frac{5083 u2}{2409} \right. \right. \\ & + \frac{6019 u5}{2409} \Big) D_{w3} \Big) dw9 + (u3 D_{w3}) dw10 - (D_{w4} dw2) + \left( \left( \frac{397 u1}{1606} - \frac{3935 u2}{4818} + \frac{5167 u5}{2409} \right) D_{w4} \right) dw7 + (u6 D_{w4}) dw8 \\ & - ((3 D_{w7} dw10) + (3 D_{w8} dw9) - ((3 D_{w9} dw6) + (3 D_{w10} dw5), \left( \left( \frac{16 u3}{117} - \frac{623 u4}{117} + \frac{16 u6}{3} \right) D_{w2} \right) dw5 \\ & - \left( \left( \left( \frac{956 u1}{2409} + \frac{164 u2}{2409} - \frac{416 u5}{2409} \right) D_{w2} \right) dw6 \right) - \left( \left( \left( \frac{20 u1}{803} - \frac{2140 u2}{2409} + \frac{2608 u5}{2409} \right) D_{w3} \right) dw5 \right) - \left( \left( \left( \frac{16 u3}{39} \right. \right. \right. \\ & + \frac{u4}{39} \Big) D_{w3} \Big) dw6 \Big) + (2 D_{w4} dw1) + \left( \left( \frac{140 u1}{803} - \frac{2132 u2}{2409} + \frac{5408 u5}{2409} \right) D_{w4} \right) dw9 + (u4 D_{w4}) dw10 - ((6 D_{w7} dw6) \\ & + (6 D_{w8} dw5) \end{aligned}$$

(7)

```
g > streqs:=cohom_algfromten(genbrak,gisoten):
```

```
g > DGsetup(LieAlgebraData(streqs,G));
```

(8)

*Lie algebra: G*

(8)

```
g > Jac:=(x,y,z)->evalDG(LieBracket(LieBracket(x,y),z)+LieBracket(LieBracket(z,x),y)+LieBracket(LieBracket(y,z),x));
```

```
Jac := (x, y, z) → DifferentialGeometry:-evalDG(DifferentialGeometry:-LieBracket(DifferentialGeometry:-LieBracket(x, y), z)  
+ DifferentialGeometry:-LieBracket(DifferentialGeometry:-LieBracket(z, x), y) + DifferentialGeometry:-  
LieBracket(DifferentialGeometry:-LieBracket(y, z), x))
```

(9)

```
g > mproj_ten:=evalDG(add(theta||i &t e||i,i=5..10));
```

$mproj\_ten := \theta_5 e_5 + \theta_6 e_6 + \theta_7 e_7 + \theta_8 e_8 + \theta_9 e_9 + \theta_{10} e_{10}$

(10)

```
g > Pm:=(x,i)->ContractIndices(mproj_ten,convert(x,DGtensor),[[1,i]]);
```

$Pm := (x, i) \rightarrow DifferentialGeometry:-Tensor:-ContractIndices(mproj\_ten, convert(x, DifferentialGeometry:-Tools:-DGtensor), [[1, i]])$

(11)

```
g > {seq(seq(seq(op(DGinfo(evalDG(convert(Jac(e||i,e||j,e||k),DGtensor) &minus Pm(Jac(e||i,e||j,e||k),1)), "CoefficientSet")), i=1..4), j=1..4), k=5..10)};
```

{0}

(12)

```
G > {seq(seq(seq(op(DGinfo(Pm(Jac(e||i,e||j,e||k),1), "CoefficientSet")), i=1..4), j=1..4), k=5..10)}
```

;

{0}

(13)

```
G > dd_eq:={seq(seq(seq(op(DGinfo(Pm(Jac(e||i,e||j,e||k),1), "CoefficientSet")), i=1..4), j=5..10), k=5..10)};
```

$dd\_eq$  are the equations  $\delta\phi = d\theta\_m$ . These are linear equations from the Jacobi system. They constrain the cohomology class  $[\phi]$ .

```
G > dd_sol:=solve(dd_eq);
```

$dd\_sol := \left\{ a_{10} = 0, a_{100} = 0, a_{105} = 0, a_{106} = 0, a_{107} = \frac{9917}{13166} u_2 - a_{69}, a_{108} = \frac{12249}{8648} u_4 - a_{70}, a_{109} = 0, a_{110} = 0, a_{115} = 0, a_{116} = 0, \right.$

(14)

$a_{117} = -\frac{211}{368} u_4 - a_{70}, a_{118} = \frac{22625}{6583} u_2 + a_{69}, a_{119} = 0, a_{120} = 0, a_{125} = 0, a_{126} = 0, a_{127} = -\frac{23189}{8648} u_4 - a_{70}, a_{128} = \frac{8789}{13166} u_2$

$+ a_{69}, a_{129} = 0, a_{130} = 0, a_{135} = 0, a_{136} = 0, a_{137} = -\frac{12813}{6583} u_2 + a_{69}, a_{138} = -\frac{187}{368} u_4 + a_{70}, a_{139} = 0, a_{140} = 0, a_{145} = 0, a_{146}$

$= 0, a_{147} = 0, a_{148} = 0, a_{149} = -\frac{371}{184} u_4, a_{15} = 0, a_{150} = -\frac{17437}{6583} u_2, a_{16} = 0, a_{17} = 0, a_{18} = 0, a_{19} = \frac{564}{6583} u_2 - a_{69}, a_{20} = -\frac{3}{46} u_4$

$- a_{70}, a_{25} = 0, a_{26} = 0, a_{27} = 0, a_{28} = 0, a_{29} = -\frac{23189}{8648} u_4 - a_{70}, a_{30} = -\frac{12813}{6583} u_2 + a_{69}, a_{35} = \frac{30709}{13166} u_2 + a_{69}, a_{36} = \frac{20313}{8648} u_4$

$+ a_{70}, a_{37} = 0, a_{38} = 0, a_{39} = 0, a_{40} = 0, a_{45} = -\frac{20333}{17296} u_4 + a_{70}, a_{46} = \frac{15125}{6583} u_2 - a_{69}, a_{47} = 0, a_{48} = 0, a_{49} = 0, a_5 = 0, a_{50} = 0,$

$$\begin{aligned}
& a_{55}=0, a_{56}=0, a_{57}=0, a_{58}=0, a_{59}=\frac{12249}{8648} u_4 - a_{70}, a_6=0, a_{60}=\frac{22625}{6583} u_2 + a_{69}, a_{65}=0, a_{66}=0, a_{67}=0, a_{68}=0, a_{69}=a_{69}, \\
& a_7=0, a_{70}=a_{70}, a_{75}=-\frac{14561}{8648} u_4 + a_{70}, a_{76}=\frac{21461}{13166} u_2 - a_{69}, a_{77}=0, a_{78}=0, a_{79}=0, a_8=0, a_{80}=0, a_{85}=-3 u_2 - a_{69}, a_{86}= \\
& -\frac{31837}{17296} u_4 - a_{70}, a_{87}=0, a_{88}=0, a_{89}=0, a_9=0, a_{90}=0, a_{95}=0, a_{96}=0, a_{97}=0, a_{98}=0, a_{99}=0, u_1=-\frac{43683}{6583} u_2, u_2=u_2, u_3 \\
& =\frac{21461}{17296} u_4, u_4=u_4, u_5=\frac{4271}{13166} u_2, u_6=\frac{23189}{17296} u_4 \}
\end{aligned}$$

The only cohomology parameters left are  $u_2$  and  $u_4$ . Use this solution to reinitialize the algebra.

```

G > newgisoten:=DGsimplify(subs(dd_sol,gisoten)):newgenbrak:=DGsimplify(subs(dd_sol,genbrak)):
g > streqs:=cohom_algfromten(newgenbrak,newgisoten):
g > DGsetup(LieAlgebraData(streqs,G));

```

*Lie algebra: G*

(15)

```

G > q_eqs:={seq(seq(seq(op(DGinfo(evalDG(convert(Jac(e||i,e||j,e||k),DGtensor) &minus Pm(Jac
(e||i,e||j,e||k),1)), "CoefficientSet")),i=1..4),j=5..10),k=5..10)}:

```

$q\_eqs$  are the equations for  $[Q(\phi)]=0$ , the final cohomological constraint on  $\phi$ . These are equations from the Jacobi system, but non-linear.

```

G > q_eqs_groebner:=Groebner[Basis](q_eqs,'tord');

```

$$\begin{aligned}
q\_eqs\_groebner:= & [a_4, a_2, a_3, a_{91}, a_{34}, a_{44}, a_{74}, a_{84}, a_{33}, a_{42}, a_{72}, a_{83}, a_{93}, a_{32}, a_{43}, a_{73}, a_{82}, a_{13}, a_{63}, a_{92}, a_{24}, a_{54}, a_{12}, a_{14}, a_{62}, \\
& a_{64}, a_{22}, a_{23}, a_{52}, a_{53}, a_{101}, a_{111}, a_{121}, a_{131}, a_1, a_{31}, a_{41}, a_{71}, a_{81}, a_{104}, a_{114}, a_{124}, a_{134}, a_{144}, a_{142}, a_{143}, a_{133} + a_{103}, \\
& 234187 a_{112} - 756564 a_{103}, 234187 a_{122} - 756564 a_{103}, a_{141}, 468374 a_{21} - 242539 a_{103}, 468374 a_{51} - 242539 a_{103}, 242539 a_{123} \\
& - 468374 a_{61}, 242539 a_{113} - 468374 a_{61}, 242539 a_{132} - 1513128 a_{61}, 242539 a_{102} + 1513128 a_{61}, a_{11} + a_{61}, a_{94}, 22798666 u_2^2 \\
& - 43335889 a_{61}, 234187 u_2 u_4 - 302818 a_{103}, 242539 u_4^2 + 795616 a_{61}, 1596634237 a_{103} u_4 + 4050498352 a_{61} u_2, \\
& -1048738636 a_{103} u_2 + 1541653021 a_{61} u_4, 1541653021 a_{69} u_4 + 2025249176 a_{70} u_2 + 1571019784 a_{103}, -1617176 a_{69} u_2 \\
& + 1231021 a_{70} u_4 - 2422544 a_{61}, 58825166521 a_{103}^2 + 219374203876 a_{61}^2, -1596634237 a_{103} a_{70} + 3083306042 a_{61} a_{69} \\
& + 2429924312 a_{61} u_2, 1596634237 a_{103} a_{69} + 1258292332 a_{103} u_2 + 3083306042 a_{61} a_{70}, 2058269543 a_{69}^2 u_2 \\
& + 2058269543 a_{70}^2 u_2 + 3193268474 a_{103} a_{70} - 2429924312 a_{61} u_2, 57857987 a_{103} a_{69}^2 + 91194664 a_{103} a_{69} u_2 \\
& + 57857987 a_{103} a_{70}^2 + 68305208 a_{103} a_{61}]
\end{aligned}$$

(16)

```

G > q_eqs_2:={op(subs(solve(q_eqs_groebner[1..58]),q_eqs_groebner))};

```

$$q\_eqs\_2:=\{0, 58825166521 a_{103}^2 + 219374203876 a_{61}^2, 22798666 u_2^2 - 43335889 a_{61}, 242539 u_4^2 + 795616 a_{61}, 234187 u_2 u_4$$

(17)

$-302818 a_{103}, 1596634237 a_{103} u_4 + 4050498352 a_{61} u_2, -1048738636 a_{103} u_2 + 1541653021 a_{61} u_4, -1596634237 a_{103} a_{70}$   
 $+ 3083306042 a_{61} a_{69} + 2429924312 a_{61} u_2, 1596634237 a_{103} a_{69} + 1258292332 a_{103} u_2 + 3083306042 a_{61} a_{70},$   
 $1541653021 a_{69} u_4 + 2025249176 a_{70} u_2 + 1571019784 a_{103}, -1617176 a_{69} u_2 + 1231021 a_{70} u_4 - 2422544 a_{61},$   
 $2058269543 a_{69}^2 u_2 + 2058269543 a_{70}^2 u_2 + 3193268474 a_{103} a_{70} - 2429924312 a_{61} u_2, 57857987 a_{103} a_{69}^2$   
 $+ 91194664 a_{103} a_{69} u_2 + 57857987 a_{103} a_{70}^2 + 68305208 a_{103} a_{61}\}$

We solve the linear equations in the Groebner basis of  $q\_eqs$ , and produce a Groebner basis of the resulting system.

```
G > {op(Groebner[Basis](q_eqs_2,'tord'))};
```

$\{58825166521 a_{103}^2 + 219374203876 a_{61}^2, 22798666 u_2^2 - 43335889 a_{61}, 242539 u_4^2 + 795616 a_{61}, 234187 u_2 u_4 - 302818 a_{103},$   
 $1596634237 a_{103} u_4 + 4050498352 a_{61} u_2, 1048738636 a_{103} u_2 - 1541653021 a_{61} u_4, 524369318 a_{103} a_{70} + 314573083 a_{103} u_4$   
 $- 1012624588 a_{61} a_{69}, 262184659 a_{103} a_{69} + 506312294 a_{61} a_{70} + 303740539 a_{61} u_4, 1541653021 a_{69} u_4 + 2025249176 a_{70} u_2$   
 $+ 1571019784 a_{103}, 1617176 a_{69} u_2 - 1231021 a_{70} u_4 + 2422544 a_{61}, 2058269543 a_{69}^2 u_4 + 2058269543 a_{70}^2 u_4$   
 $+ 4194954544 a_{103} a_{69} + 2429924312 a_{61} u_4\}$

Since we are working over the real numbers, sums of squares must vanish identically. Therefore  $a_{103}=a_{11}=0$ .

```
G > subs({a103=0,a11=0},{op(Groebner[Basis](q_eqs_2,'tord'))});
```

$\{219374203876 a_{61}^2, 4050498352 a_{61} u_2, -1541653021 a_{61} u_4, -1012624588 a_{69} a_{61}, 234187 u_2 u_4, 22798666 u_2^2 - 43335889 a_{61},$   
 $242539 u_4^2 + 795616 a_{61}, 506312294 a_{61} a_{70} + 303740539 a_{61} u_4, 1541653021 a_{69} u_4 + 2025249176 a_{70} u_2, 2058269543 a_{69}^2 u_4$   
 $+ 2058269543 a_{70}^2 u_4 + 2429924312 a_{61} u_4, 1617176 a_{69} u_2 - 1231021 a_{70} u_4 + 2422544 a_{61}\}$

This implies that the last cohomology parameters  $u_2, u_4$  vanish, hence  $[\phi]=0$ , which is what we wanted to show in this section.

## Section 2: $h=1_0$

We import the representation matrices from the other worksheet. In this case, the cohomology is 10D.

```
V > MrepMat := [Matrix(9, 9, {(1, 1) = 0, (1, 2) = 0, (1, 3) = 0, (1, 4) = (1/7)*u7-(19/7)*u8-
(24/7)*u9, (1, 5) = (9/5)*u5-(19/15)*u6-(21/5)*u10, (1, 6) = 0, (1, 7) = 0, (1, 8) = -(55/39)
*u2+(4243/1833)*u3, (1, 9) = u4, (2, 1) = 0, (2, 2) = 0, (2, 3) = 0, (2, 4) = u6, (2, 5) =
(24/7)*u7-(15/7)*u8-(9/7)*u9, (2, 6) = 0, (2, 7) = 0, (2, 8) = u1, (2, 9) = -(55/117)*u2-
(1/117)*u3, (3, 1) = 0, (3, 2) = 1, (3, 3) = 0, (3, 4) = 0, (3, 5) = 0, (3, 6) = (389/6050)*
u1+(423/6050)*u4, (3, 7) = (8/117)*u2-(19/117)*u3, (3, 8) = -u6-3*u10, (3, 9) = -(3/7)*u7+
(15/7)*u8+(9/7)*u9, (4, 1) = 0, (4, 2) = 0, (4, 3) = 0, (4, 4) = 0, (4, 5) = 0, (4, 6) = 0,
(4, 7) = 0, (4, 8) = 0, (4, 9) = 0, (5, 1) = 0, (5, 2) = 0, (5, 3) = 0, (5, 4) = 0, (5, 5) =
```

```

0, (5, 6) = 0, (5, 7) = 0, (5, 8) = 0, (5, 9) = 0, (6, 1) = 0, (6, 2) = 0, (6, 3) = 0, (6, 4)
= 0, (6, 5) = 0, (6, 6) = 0, (6, 7) = 0, (6, 8) = 1, (6, 9) = 0, (7, 1) = 0, (7, 2) = 0, (7,
3) = 0, (7, 4) = 0, (7, 5) = 0, (7, 6) = 0, (7, 7) = 0, (7, 8) = 0, (7, 9) = 1, (8, 1) = 0,
(8, 2) = 0, (8, 3) = 0, (8, 4) = -1, (8, 5) = 0, (8, 6) = 0, (8, 7) = 0, (8, 8) = 0, (8, 9) =
0, (9, 1) = 0, (9, 2) = 0, (9, 3) = 0, (9, 4) = 0, (9, 5) = -1, (9, 6) = 0, (9, 7) = 0, (9,
8) = 0, (9, 9) = 0}}, Matrix(9, 9, {(1, 1) = 0, (1, 2) = 0, (1, 3) = 0, (1, 4) = u5, (1, 5) =
u9, (1, 6) = 0, (1, 7) = 0, (1, 8) = -(423/6050)*u1-(13011/6050)*u4, (1, 9) = -3*u2+(234/47)*
u3, (2, 1) = 0, (2, 2) = 0, (2, 3) = 0, (2, 4) = u7, (2, 5) = u10, (2, 6) = 0, (2, 7) = 0,
(2, 8) = u2, (2, 9) = (12729/6050)*u1-(47/6050)*u4, (3, 1) = -1, (3, 2) = 0, (3, 3) = 0, (3,
4) = 0, (3, 5) = 0, (3, 6) = -(8/39)*u2+(1517/1833)*u3, (3, 7) = (3807/6050)*u1+(2149/6050)*
u4, (3, 8) = (1/7)*u7-(19/7)*u8-(3/7)*u9, (3, 9) = -(6/5)*u5-(19/15)*u6-(21/5)*u10, (4, 1) =
0, (4, 2) = 0, (4, 3) = 0, (4, 4) = 0, (4, 5) = 0, (4, 6) = 0, (4, 7) = 0, (4, 8) = 0, (4, 9)
= 0, (5, 1) = 0, (5, 2) = 0, (5, 3) = 0, (5, 4) = 0, (5, 5) = 0, (5, 6) = 0, (5, 7) = 0, (5,
8) = 0, (5, 9) = 0, (6, 1) = 0, (6, 2) = 0, (6, 3) = 0, (6, 4) = 0, (6, 5) = 0, (6, 6) = 0,
(6, 7) = 0, (6, 8) = 0, (6, 9) = -3, (7, 1) = 0, (7, 2) = 0, (7, 3) = 0, (7, 4) = 0, (7, 5) =
0, (7, 6) = 0, (7, 7) = 0, (7, 8) = 3, (7, 9) = 0, (8, 1) = 0, (8, 2) = 0, (8, 3) = 0, (8, 4)
= 0, (8, 5) = -3, (8, 6) = 0, (8, 7) = 0, (8, 8) = 0, (8, 9) = 0, (9, 1) = 0, (9, 2) = 0, (9,
3) = 0, (9, 4) = 3, (9, 5) = 0, (9, 6) = 0, (9, 7) = 0, (9, 8) = 0, (9, 9) = 0}}, Matrix(9,
9, {(1, 1) = 0, (1, 2) = 0, (1, 3) = 0, (1, 4) = -(423/6050)*u1+(5139/6050)*u4, (1, 5) =
(16/13)*u2-(1201/611)*u3, (1, 6) = 0, (1, 7) = 0, (1, 8) = 0, (1, 9) = 0, (2, 1) = 0, (2, 2)
= 0, (2, 3) = 0, (2, 4) = -(16/39)*u2-(1/39)*u3, (2, 5) = -(5421/6050)*u1-(47/6050)*u4, (2,
6) = 0, (2, 7) = 0, (2, 8) = 0, (2, 9) = 0, (3, 1) = 0, (3, 2) = 0, (3, 3) = 0, (3, 4) = u8,
(3, 5) = (3/5)*u5+(7/15)*u6+(8/5)*u10, (3, 6) = 0, (3, 7) = 0, (3, 8) = u3, (3, 9) =
(141/110)*u1+(47/110)*u4, (4, 1) = 0, (4, 2) = 0, (4, 3) = 0, (4, 4) = 0, (4, 5) = 0, (4, 6)
= 0, (4, 7) = 0, (4, 8) = 0, (4, 9) = 0, (5, 1) = 0, (5, 2) = 0, (5, 3) = 0, (5, 4) = 0, (5,
5) = 0, (5, 6) = 0, (5, 7) = 0, (5, 8) = 0, (5, 9) = 0, (6, 1) = 0, (6, 2) = 0, (6, 3) = 0,
(6, 4) = 0, (6, 5) = -6, (6, 6) = 0, (6, 7) = 0, (6, 8) = 0, (6, 9) = 0, (7, 1) = 0, (7, 2) =
0, (7, 3) = 0, (7, 4) = 6, (7, 5) = 0, (7, 6) = 0, (7, 7) = 0, (7, 8) = 0, (7, 9) = 0, (8, 1)
= 0, (8, 2) = 0, (8, 3) = 0, (8, 4) = 0, (8, 5) = 0, (8, 6) = 0, (8, 7) = 0, (8, 8) = 0, (8,
9) = 0, (9, 1) = 0, (9, 2) = 0, (9, 3) = 0, (9, 4) = 0, (9, 5) = 0, (9, 6) = 0, (9, 7) = 0,
(9, 8) = 0, (9, 9) = 0}}]);

```

For some reason Maple has a hard time computing the structure constants from these matrices, so we enter them manually.

```
V80 > HData:=LieAlgebraData([[t1,t2]=t3],[t1,t2,t3],h):DGsetup(HData);
```

*Lie algebra: h*

(20)

```
V > DGsetup([seq(v||i,i=1..dimM)],m);
```

*frame name: m*

(21)

```
m > DGsetup([seq(w||i,i=1..9)],g);
```

*frame name: g*

(22)



```
g > rep:=Representation(h,g,MrepMat):
G > ChangeFrame(g);
```

g

(23)

```
g > L2M:=GenerateForms(DGinfo(g,"FrameBaseForms")[4..9],2);
```

```
L2M:=[dw4 ∧ dw5, dw4 ∧ dw6, dw4 ∧ dw7, dw4 ∧ dw8, dw4 ∧ dw9, dw5 ∧ dw6, dw5 ∧ dw7, dw5 ∧ dw8, dw5 ∧ dw9, dw6 ∧ dw7,
dw6 ∧ dw8, dw6 ∧ dw9, dw7 ∧ dw8, dw7 ∧ dw9, dw8 ∧ dw9]
```

(24)

```
g > brakspace:=GenerateTensors([L2M,DGinfo(g,"FrameBaseVectors")]):
```

```
g > genbrak:=evalDG(add(a||i*brakspace[i],i=1..nops(brakspace))):
```

```
g > gisoten:=map(x->convert(x,DGtensor,["con_bas", "cov_bas"], []),MrepMat);
```

```
gisoten := [ ( ( (  $\frac{u7}{7} - \frac{19u8}{7} - \frac{24u9}{7}$  )  $D_{w1}$  )  $dw4 - ( ( ( -\frac{9u5}{5} + \frac{19u6}{15} + \frac{21u10}{5}$  )  $D_{w1}$  )  $dw5 - ( ( ( \frac{55u2}{39}$ 
-  $\frac{4243u3}{1833}$  )  $D_{w1}$  )  $dw8$  ) +  $(u4 D_{w1}) dw9 + (u6 D_{w2}) dw4 + ( ( \frac{24u7}{7} - \frac{15u8}{7} - \frac{9u9}{7}$  )  $D_{w2}$  )  $dw5 + (u1 D_{w2}) dw8$ 
- ( ( (  $\frac{55u2}{117} + \frac{u3}{117}$  )  $D_{w2}$  )  $dw9$  ) +  $D_{w3} dw2 + ( ( \frac{389u1}{6050} + \frac{423u4}{6050}$  )  $D_{w3}$  )  $dw6 + ( ( \frac{8u2}{117} - \frac{19u3}{117}$  )  $D_{w3}$  )  $dw7$ 
- ( ( (  $(u6 + 3u10) D_{w3}$  )  $dw8$  ) - ( ( (  $\frac{3u7}{7} - \frac{15u8}{7} - \frac{9u9}{7}$  )  $D_{w3}$  )  $dw9$  ) +  $D_{w6} dw8 + D_{w7} dw9 - (D_{w8} dw4)$ 
-  $(D_{w9} dw5), (u5 D_{w1}) dw4 + (u9 D_{w1}) dw5 - ( ( ( \frac{423u1}{6050} + \frac{13011u4}{6050}$  )  $D_{w1}$  )  $dw8 - ( ( ( 3u2 - \frac{234u3}{47}$  )  $D_{w1}$  )  $dw9$  )
+  $(u7 D_{w2}) dw4 + (u10 D_{w2}) dw5 + (u2 D_{w2}) dw8 + ( ( \frac{12729u1}{6050} - \frac{47u4}{6050}$  )  $D_{w2}$  )  $dw9 - (D_{w3} dw1) - ( ( ( \frac{8u2}{39}$ 
-  $\frac{1517u3}{1833}$  )  $D_{w3}$  )  $dw6$  ) + ( ( (  $\frac{3807u1}{6050} + \frac{2149u4}{6050}$  )  $D_{w3}$  )  $dw7 + ( ( \frac{u7}{7} - \frac{19u8}{7} - \frac{3u9}{7}$  )  $D_{w3}$  )  $dw8 - ( ( ( \frac{6u5}{5}$ 
+  $\frac{19u6}{15} + \frac{21u10}{5}$  )  $D_{w3}$  )  $dw9$  ) - ( (  $3 D_{w6}$  )  $dw9$  ) +  $(3 D_{w7}) dw8 - ( ( 3 D_{w8}$  )  $dw5$  ) +  $(3 D_{w9}) dw4, - ( ( ( \frac{423u1}{6050}$ 
-  $\frac{5139u4}{6050}$  )  $D_{w1}$  )  $dw4$  ) + ( ( (  $\frac{16u2}{13} - \frac{1201u3}{611}$  )  $D_{w1}$  )  $dw5 - ( ( ( \frac{16u2}{39} + \frac{u3}{39}$  )  $D_{w2}$  )  $dw4$  ) - ( ( (  $\frac{5421u1}{6050}$ 
+  $\frac{47u4}{6050}$  )  $D_{w2}$  )  $dw5$  ) +  $(u8 D_{w3}) dw4 + ( ( \frac{3u5}{5} + \frac{7u6}{15} + \frac{8u10}{5}$  )  $D_{w3}$  )  $dw5 + (u3 D_{w3}) dw8 + ( ( \frac{141u1}{110}$ 
+  $\frac{47u4}{110}$  )  $D_{w3}$  )  $dw9 - ( ( 6 D_{w6}$  )  $dw5$  ) +  $(6 D_{w7}) dw4$  ]
```

(25)

```
g > streqs:=cohom_algfromten(genbrak,gisoten);
```

$$\begin{aligned}
\text{streps} := & \left[ [o1, o2] = a1 r1 + a2 r2 + a3 r3 + a4 o1 + a5 o2 + a6 o3 + a7 o4 + a8 o5 + a9 o6, [o1, o3] = a10 r1 + a11 r2 + a12 r3 + a13 o1 \right. \\
& + a14 o2 + a15 o3 + a16 o4 + a17 o5 + a18 o6, [o1, o4] = a19 r1 + a20 r2 + a21 r3 + a22 o1 + a23 o2 + a24 o3 + a25 o4 + a26 o5 \\
& + a27 o6, [o1, o5] = a28 r1 + a29 r2 + a30 r3 + a31 o1 + a32 o2 + a33 o3 + a34 o4 + a35 o5 + a36 o6, [o1, o6] = a37 r1 + a38 r2 \\
& + a39 r3 + a40 o1 + a41 o2 + a42 o3 + a43 o4 + a44 o5 + a45 o6, [o2, o3] = a46 r1 + a47 r2 + a48 r3 + a49 o1 + a50 o2 + a51 o3 \\
& + a52 o4 + a53 o5 + a54 o6, [o2, o4] = a55 r1 + a56 r2 + a57 r3 + a58 o1 + a59 o2 + a60 o3 + a61 o4 + a62 o5 + a63 o6, [o2, o5] \\
& = a64 r1 + a65 r2 + a66 r3 + a67 o1 + a68 o2 + a69 o3 + a70 o4 + a71 o5 + a72 o6, [o2, o6] = a73 r1 + a74 r2 + a75 r3 + a76 o1 \\
& + a77 o2 + a78 o3 + a79 o4 + a80 o5 + a81 o6, [o3, o4] = a82 r1 + a83 r2 + a84 r3 + a85 o1 + a86 o2 + a87 o3 + a88 o4 + a89 o5 \\
& + a90 o6, [o3, o5] = a91 r1 + a92 r2 + a93 r3 + a94 o1 + a95 o2 + a96 o3 + a97 o4 + a98 o5 + a99 o6, [o3, o6] = a100 r1 + a101 r2 \\
& + a102 r3 + a103 o1 + a104 o2 + a105 o3 + a106 o4 + a107 o5 + a108 o6, [o4, o5] = a109 r1 + a110 r2 + a111 r3 + a112 o1 \\
& + a113 o2 + a114 o3 + a115 o4 + a116 o5 + a117 o6, [o4, o6] = a118 r1 + a119 r2 + a120 r3 + a121 o1 + a122 o2 + a123 o3 \\
& + a124 o4 + a125 o5 + a126 o6, [o5, o6] = a127 r1 + a128 r2 + a129 r3 + a130 o1 + a131 o2 + a132 o3 + a133 o4 + a134 o5 \\
& + a135 o6, [r1, o1] = -o5 + \left( \frac{1}{7} u7 - \frac{19}{7} u8 - \frac{24}{7} u9 \right) r1 + u6 r2, [r1, o2] = -o6 + \left( \frac{9}{5} u5 - \frac{19}{15} u6 - \frac{21}{5} u10 \right) r1 + \left( \frac{24}{7} u7 \right. \\
& - \frac{15}{7} u8 - \frac{9}{7} u9 \left. \right) r2, [r1, o3] = \left( \frac{389}{6050} u1 + \frac{423}{6050} u4 \right) r3, [r1, o4] = \left( \frac{8}{117} u2 - \frac{19}{117} u3 \right) r3, [r1, o5] = o3 + \left( -\frac{55}{39} u2 \right. \\
& + \frac{4243}{1833} u3 \left. \right) r1 + u1 r2 + (-u6 - 3 u10) r3, [r1, o6] = o4 + u4 r1 + \left( -\frac{55}{117} u2 - \frac{1}{117} u3 \right) r2 + \left( -\frac{3}{7} u7 + \frac{15}{7} u8 + \frac{9}{7} u9 \right) r3, \\
& [r2, o1] = r1 u5 + r2 u7 + 3 o6, [r2, o2] = r1 u9 + r2 u10 - 3 o5, [r2, o3] = \left( -\frac{8}{39} u2 + \frac{1517}{1833} u3 \right) r3, [r2, o4] = \left( \frac{3807}{6050} u1 \right.
\end{aligned}
\tag{26}$$

$$\begin{aligned}
& + \frac{2149}{6050} u_4 \Big) r_3, [r_2, o_5] = 3 o_4 + \left( -\frac{423}{6050} u_1 - \frac{13011}{6050} u_4 \right) r_1 + u_2 r_2 + \left( \frac{1}{7} u_7 - \frac{19}{7} u_8 - \frac{3}{7} u_9 \right) r_3, [r_2, o_6] = -3 o_3 + \left( -3 u_2 \right. \\
& + \frac{234}{47} u_3 \Big) r_1 + \left( \frac{12729}{6050} u_1 - \frac{47}{6050} u_4 \right) r_2 + \left( -\frac{6}{5} u_5 - \frac{19}{15} u_6 - \frac{21}{5} u_{10} \right) r_3, [r_3, o_1] = 6 o_4 + \left( -\frac{423}{6050} u_1 + \frac{5139}{6050} u_4 \right) r_1 \\
& + \left( -\frac{16}{39} u_2 - \frac{1}{39} u_3 \right) r_2 + u_8 r_3, [r_3, o_2] = -6 o_3 + \left( \frac{16}{13} u_2 - \frac{1201}{611} u_3 \right) r_1 + \left( -\frac{5421}{6050} u_1 - \frac{47}{6050} u_4 \right) r_2 + \left( \frac{3}{5} u_5 + \frac{7}{15} u_6 \right. \\
& + \frac{8}{5} u_{10} \Big) r_3, [r_3, o_3] = 0, [r_3, o_4] = 0, [r_3, o_5] = u_3 r_3, [r_3, o_6] = \left( \frac{141}{110} u_1 + \frac{47}{110} u_4 \right) r_3, [r_1, r_2] = r_3, [r_1, r_3] = 0, [r_2, r_3] = 0 \Big], \\
& [r_1, r_2, r_3, o_1, o_2, o_3, o_4, o_5, o_6]
\end{aligned}$$

**g** > DGsetup(LieAlgebraData(streqs,G));

*Lie algebra: G*

(27)

**g** > Jac:=(x,y,z)->evalDG(LieBracket(LieBracket(x,y),z)+LieBracket(LieBracket(z,x),y)+LieBracket(LieBracket(y,z),x));

*Jac := (x, y, z) → DifferentialGeometry:-evalDG(DifferentialGeometry:-LieBracket(DifferentialGeometry:-LieBracket(x, y), z) + DifferentialGeometry:-LieBracket(DifferentialGeometry:-LieBracket(z, x), y) + DifferentialGeometry:-LieBracket(DifferentialGeometry:-LieBracket(y, z), x))*

(28)

**g** > mproj\_ten:=evalDG(add(theta||i &t e||i,i=4..9));

*mproj\_ten := θ4 e4 + θ5 e5 + θ6 e6 + θ7 e7 + θ8 e8 + θ9 e9*

(29)

**g** > Pm:=(x,i)->ContractIndices(mproj\_ten,convert(x,DGtensor),[[1,i]]);

*Pm := (x, i) → DifferentialGeometry:-Tensor.-ContractIndices(mproj\_ten, convert(x, DifferentialGeometry:-Tools:-DGtensor), [[1, i]])*

(30)

**g** > {seq(seq(seq(op(DGinfo(evalDG(convert(Jac(e||i,e||j,e||k),DGtensor) &minus Pm(Jac(e||i,e||j,e||k),1)), "CoefficientSet")),i=1..3),j=1..3),k=4..9)};

*{0}*

(31)

**G** > {seq(seq(seq(op(DGinfo(Pm(Jac(e||i,e||j,e||k),1), "CoefficientSet")),i=1..3),j=1..3),k=4..9)};

*{0}*

(32)

**G** > dd\_eq:={seq(seq(seq(op(DGinfo(Pm(Jac(e||i,e||j,e||k),1), "CoefficientSet")),i=1..3),j=4..9),k=4..9)};

**G** > dd\_sol:=solve(dd\_eq);nops(%);

*dd\_sol := {a103=0, a104=0, a105 =  $\frac{2}{109} u_4 - a63$ , a106 =  $-\frac{63}{47} u_3 + a62$ , a107=0, a108=0, a112=0, a113=0, a114 =  $-\frac{124}{109} u_4$*

*- a63, a115 = a62, a116=0, a117=0, a121=0, a122=0, a123 =  $\frac{30}{47} u_3 + a62$ , a124 = a63, a125=0, a126=0, a13=0, a130=0, a131*

$$\begin{aligned}
&=0, a_{132}=a_{132}, a_{133}=a_{133}, a_{134}=-\frac{94}{109}u_4, a_{135}=u_3, a_{14}=0, a_{15}=\frac{2273}{1365}u_9+a_{35}, a_{16}=-\frac{457}{271}u_6-a_4-a_{81}, a_{17}=\frac{1}{47}u_3 \\
&-a_{62}, a_{18}=\frac{2}{109}u_4-a_{63}, a_{22}=0, a_{23}=0, a_{24}=-\frac{289}{813}u_6+a_{132}+a_4+a_{81}, a_{25}=a_{133}+a_{35}+\frac{1311}{455}u_9, a_{26}=-\frac{124}{109}u_4 \\
&-a_{63}, a_{27}=\frac{30}{47}u_3+a_{62}, a_{31}=-\frac{111}{94}u_3+a_{62}, a_{32}=a_{63}+u_4, a_{33}=a_{33}, a_{34}=a_{34}, a_{35}=a_{35}, a_{36}=\frac{248}{271}u_6-a_4-a_{81}, a_4 \\
&=a_4, a_{40}=-\frac{79}{109}u_4+a_{63}, a_{41}=-\frac{77}{94}u_3-a_{62}, a_{42}=a_{42}, a_{43}=a_{43}, a_{44}=-\frac{2728}{813}u_6+a_4+a_{81}, a_{45}=\frac{1984}{1365}u_9+a_{35}, a_{49} \\
&=0, a_5=-a_{72}-\frac{2728}{1365}u_9+a_{35}, a_{50}=0, a_{51}=\frac{1311}{271}u_6-a_{132}+a_{81}, a_{52}=-a_{133}+a_{72}+\frac{813}{455}u_9, a_{53}=\frac{62}{109}u_4-a_{63}, a_{54}= \\
&-\frac{63}{47}u_3+a_{62}, a_{58}=0, a_{59}=0, a_{60}=-a_{72}-\frac{4099}{1365}u_9, a_{61}=\frac{2273}{813}u_6+a_{81}, a_{62}=a_{62}, a_{63}=a_{63}, a_{67}=-\frac{79}{109}u_4+a_{63}, a_{68}= \\
&-\frac{77}{94}u_3-a_{62}, a_{69}=a_{42}+a_8, a_{70}=a_{43}+a_9, a_{71}=\frac{1984}{813}u_6+a_{81}, a_{72}=a_{72}, a_{76}=\frac{111}{94}u_3-a_{62}, a_{77}=-u_4-a_{63}, a_{78}=-a_{33} \\
&+a_9, a_{79}=-a_{34}-a_8, a_8=a_8, a_{80}=-a_{72}-\frac{1984}{1365}u_9, a_{81}=a_{81}, a_{85}=0, a_{86}=0, a_{87}=0, a_{88}=0, a_{89}=0, a_9=a_9, a_{90}=0, a_{94} \\
&=0, a_{95}=0, a_{96}=\frac{1}{47}u_3-a_{62}, a_{97}=\frac{62}{109}u_4-a_{63}, a_{98}=0, a_{99}=0, u_1=\frac{37}{109}u_4, u_{10}=-\frac{289}{813}u_6, u_2=\frac{77}{94}u_3, u_3=u_3, u_4=u_4, \\
&u_5=-\frac{455}{271}u_6, u_6=u_6, u_7=-\frac{289}{1365}u_9, u_8=-\frac{902}{1365}u_9, u_9=u_9 \}
\end{aligned}$$

98

(33)

```

g > genbrak:=subs(dd_sol,genbrak):
g > gisoten:=subs(dd_sol,gisoten):
g > streqs:=cohom_alfromten(genbrak,gisoten);

```

$$\begin{aligned}
\text{streqs} &:= \left[ [o1, o2] = a_4 o1 + \left( -a_{72} - \frac{2728}{1365}u_9 + a_{35} \right) o2 + a_6 o3 + a_7 o4 + a_8 o5 + a_9 o6 + a_{10} r1 + a_{11} r2 + a_{12} r3, [o1, o3] \right. \\
&= \left( \frac{2273}{1365}u_9 + a_{35} \right) o3 + \left( -\frac{457}{271}u_6 - a_4 - a_{81} \right) o4 + \left( \frac{1}{47}u_3 - a_{62} \right) o5 + \left( \frac{2}{109}u_4 - a_{63} \right) o6 + a_{10} r1 + a_{11} r2 + a_{12} r3, \\
&[o1, o4] = \left( -\frac{289}{813}u_6 + a_{132} + a_4 + a_{81} \right) o3 + \left( a_{133} + a_{35} + \frac{1311}{455}u_9 \right) o4 + \left( -\frac{124}{109}u_4 - a_{63} \right) o5 + \left( \frac{30}{47}u_3 + a_{62} \right) o6
\end{aligned}$$

(34)

$$\begin{aligned}
& + a_{19} r_1 + a_{20} r_2 + a_{21} r_3, [o_1, o_5] = \left( -\frac{111}{94} u_3 + a_{62} \right) o_1 + (a_{63} + u_4) o_2 + a_{33} o_3 + a_{34} o_4 + a_{35} o_5 + \left( \frac{248}{271} u_6 - a_4 \right. \\
& \left. - a_{81} \right) o_6 + a_{28} r_1 + a_{29} r_2 + a_{30} r_3, [o_1, o_6] = \left( -\frac{79}{109} u_4 + a_{63} \right) o_1 + \left( -\frac{77}{94} u_3 - a_{62} \right) o_2 + a_{42} o_3 + a_{43} o_4 + \left( -\frac{2728}{813} u_6 \right. \\
& \left. + a_4 + a_{81} \right) o_5 + \left( \frac{1984}{1365} u_9 + a_{35} \right) o_6 + a_{37} r_1 + a_{38} r_2 + a_{39} r_3, [o_2, o_3] = \left( \frac{1311}{271} u_6 - a_{132} + a_{81} \right) o_3 + \left( -a_{133} + a_{72} \right. \\
& \left. + \frac{813}{455} u_9 \right) o_4 + \left( \frac{62}{109} u_4 - a_{63} \right) o_5 + \left( -\frac{63}{47} u_3 + a_{62} \right) o_6 + a_{46} r_1 + a_{47} r_2 + a_{48} r_3, [o_2, o_4] = \left( -a_{72} - \frac{4099}{1365} u_9 \right) o_3 \\
& + \left( \frac{2273}{813} u_6 + a_{81} \right) o_4 + a_{62} o_5 + a_{63} o_6 + a_{55} r_1 + a_{56} r_2 + a_{57} r_3, [o_2, o_5] = \left( -\frac{79}{109} u_4 + a_{63} \right) o_1 + \left( -\frac{77}{94} u_3 - a_{62} \right) o_2 \\
& + (a_{42} + a_8) o_3 + (a_{43} + a_9) o_4 + \left( \frac{1984}{813} u_6 + a_{81} \right) o_5 + a_{72} o_6 + a_{64} r_1 + a_{65} r_2 + a_{66} r_3, [o_2, o_6] = \left( \frac{111}{94} u_3 - a_{62} \right) o_1 + ( \\
& -u_4 - a_{63}) o_2 + (-a_{33} + a_9) o_3 + (-a_{34} - a_8) o_4 + \left( -a_{72} - \frac{1984}{1365} u_9 \right) o_5 + a_{81} o_6 + a_{73} r_1 + a_{74} r_2 + a_{75} r_3, [o_3, o_4] = a_{82} r_1 \\
& + a_{83} r_2 + a_{84} r_3, [o_3, o_5] = \left( \frac{1}{47} u_3 - a_{62} \right) o_3 + \left( \frac{62}{109} u_4 - a_{63} \right) o_4 + a_{91} r_1 + a_{92} r_2 + a_{93} r_3, [o_3, o_6] = \left( \frac{2}{109} u_4 - a_{63} \right) o_3 \\
& + \left( -\frac{63}{47} u_3 + a_{62} \right) o_4 + a_{100} r_1 + a_{101} r_2 + a_{102} r_3, [o_4, o_5] = \left( -\frac{124}{109} u_4 - a_{63} \right) o_3 + a_{62} o_4 + a_{109} r_1 + a_{110} r_2 + a_{111} r_3, \\
& [o_4, o_6] = \left( \frac{30}{47} u_3 + a_{62} \right) o_3 + a_{63} o_4 + a_{118} r_1 + a_{119} r_2 + a_{120} r_3, [o_5, o_6] = a_{132} o_3 + a_{133} o_4 - \frac{94}{109} u_4 o_5 + u_3 o_6 + a_{127} r_1 \\
& + a_{128} r_2 + a_{129} r_3, [r_1, o_1] = -o_5 - \frac{2273}{1365} u_9 r_1 + u_6 r_2, [r_1, o_2] = -o_6 - \frac{2273}{813} u_6 r_1 - \frac{271}{455} u_9 r_2, [r_1, o_3] = \frac{10}{109} u_4 r_3, [r_1, o_4] \\
& = -\frac{5}{47} u_3 r_3, [r_1, o_5] = o_3 + \frac{109}{94} u_3 r_1 + \frac{37}{109} u_4 r_2 + \frac{18}{271} u_6 r_3, [r_1, o_6] = o_4 + u_4 r_1 - \frac{37}{94} u_3 r_2 - \frac{18}{455} u_9 r_3, [r_2, o_1] = 3 o_6 \\
& - \frac{455}{271} u_6 r_1 - \frac{289}{1365} u_9 r_2, [r_2, o_2] = -3 o_5 + u_9 r_1 - \frac{289}{813} u_6 r_2, [r_2, o_3] = \frac{31}{47} u_3 r_3, [r_2, o_4] = \frac{62}{109} u_4 r_3, [r_2, o_5] = 3 o_4 \\
& - \frac{237}{109} u_4 r_1 + \frac{77}{94} u_3 r_2 + \frac{1822}{1365} u_9 r_3, [r_2, o_6] = -3 o_3 + \frac{237}{94} u_3 r_1 + \frac{77}{109} u_4 r_2 + \frac{1822}{813} u_6 r_3, [r_3, o_1] = 6 o_4 + \frac{90}{109} u_4 r_1 \\
& - \frac{17}{47} u_3 r_2 - \frac{902}{1365} u_9 r_3, [r_3, o_2] = -6 o_3 - \frac{45}{47} u_3 r_1 - \frac{34}{109} u_4 r_2 - \frac{902}{813} u_6 r_3, [r_3, o_3] = 0, [r_3, o_4] = 0, [r_3, o_5] = u_3 r_3, [r_3,
\end{aligned}$$



$$\begin{aligned}
& + 8 a63 \bigg) \vartheta4 \bigg) \vartheta9 \bigg) e4 - \bigg( \bigg( \bigg( \bigg( \frac{120 u4}{109} + 8 a63 \bigg) \vartheta4 \bigg) \vartheta7 \bigg) e8 \bigg) + \bigg( \bigg( \bigg( -\frac{68 u3}{47} + 8 a62 \bigg) \vartheta9 \bigg) \vartheta5 \bigg) e4 - \bigg( \bigg( \bigg( \bigg( \frac{120 u4}{109} \\
& + 8 a63 \bigg) \vartheta9 \bigg) \vartheta4 \bigg) e4 \bigg) - \bigg( \bigg( \bigg( \bigg( -\frac{68 u3}{47} + 8 a62 \bigg) \vartheta8 \bigg) \vartheta7 \bigg) e7 \bigg) + \bigg( \bigg( \bigg( \bigg( \frac{120 u4}{109} + 8 a63 \bigg) \vartheta8 \bigg) \vartheta7 \bigg) e6 + \bigg( \bigg( \bigg( \bigg( \frac{120 u4}{109} \\
& + 8 a63 \bigg) \vartheta8 \bigg) \vartheta6 \bigg) e7 + \bigg( \bigg( (4 a42 + 4 a34 + 4 a8) \vartheta4 \bigg) \vartheta8 \bigg) e7 + \bigg( \bigg( \bigg( -\frac{68 u3}{47} + 8 a62 \bigg) \vartheta8 \bigg) \vartheta6 \bigg) e6 + \bigg( \bigg( (4 a33 - 4 a9 \\
& - 4 a43) \vartheta8 \bigg) \vartheta5 \bigg) e7 - \bigg( \bigg( \bigg( (4 a42 + 4 a34 + 4 a8) \vartheta8 \bigg) \vartheta5 \bigg) e6 \bigg) + \bigg( \bigg( \bigg( -\frac{68 u3}{47} + 8 a62 \bigg) \vartheta8 \bigg) \vartheta5 \bigg) e5 - \bigg( \bigg( \bigg( \bigg( \frac{120 u4}{109} \\
& + 8 a63 \bigg) \vartheta8 \bigg) \vartheta5 \bigg) e4 \bigg) - \bigg( \bigg( \bigg( (4 a42 + 4 a34 + 4 a8) \vartheta8 \bigg) \vartheta4 \bigg) e7 \bigg) + \bigg( \bigg( (4 a42 + 4 a34 + 4 a8) \vartheta9 \bigg) \vartheta5 \bigg) e7 - \bigg( \bigg( \bigg( (4 a33 - 4 a9 \\
& - 4 a43) \vartheta8 \bigg) \vartheta4 \bigg) e6 \bigg) - \bigg( \bigg( \bigg( (4 a33 - 4 a9 - 4 a43) \vartheta4 \bigg) \vartheta9 \bigg) e7 \bigg) - \bigg( \bigg( \bigg( \bigg( \frac{120 u4}{109} + 8 a63 \bigg) \vartheta8 \bigg) \vartheta4 \bigg) e5 \bigg) - \bigg( \bigg( \bigg( \bigg( -\frac{68 u3}{47} \\
& + 8 a62 \bigg) \vartheta8 \bigg) \vartheta4 \bigg) e4 \bigg) + \bigg( \bigg( \bigg( \bigg( \frac{120 u4}{109} + 8 a63 \bigg) \vartheta7 \bigg) \vartheta9 \bigg) e7 - \bigg( \bigg( \bigg( \bigg( -\frac{68 u3}{47} + 8 a62 \bigg) \vartheta4 \bigg) \vartheta6 \bigg) e8 \bigg) + \bigg( \bigg( \bigg( \bigg( \frac{120 u4}{109} \\
& + 8 a63 \bigg) \vartheta4 \bigg) \vartheta8 \bigg) e5 + \bigg( \bigg( \bigg( \bigg( -\frac{68 u3}{47} + 8 a62 \bigg) \vartheta7 \bigg) \vartheta9 \bigg) e6 + \bigg( \bigg( \bigg( \bigg( \frac{120 u4}{109} + 8 a63 \bigg) \vartheta9 \bigg) \vartheta5 \bigg) e5 - \bigg( \bigg( \bigg( \bigg( -\frac{68 u3}{47} \\
& + 8 a62 \bigg) \vartheta9 \bigg) \vartheta6 \bigg) e7 \bigg) + \bigg( \bigg( \bigg( \bigg( -\frac{68 u3}{47} + 8 a62 \bigg) \vartheta7 \bigg) \vartheta8 \bigg) e7 - \bigg( \bigg( \bigg( (4 a42 + 4 a34 + 4 a8) \vartheta9 \bigg) \vartheta4 \bigg) e6 \bigg) - \bigg( \bigg( \bigg( \bigg( \frac{120 u4}{109} \\
& + 8 a63 \bigg) \vartheta7 \bigg) \vartheta8 \bigg) e6 \bigg) - \bigg( \bigg( \bigg( \bigg( \bigg( \frac{120 u4}{109} + 8 a63 \bigg) \vartheta7 \bigg) \vartheta5 \bigg) e9 \bigg) + \bigg( \bigg( (4 a33 - 4 a9 - 4 a43) \vartheta4 \bigg) \vartheta8 \bigg) e6 - \bigg( \bigg( \bigg( \bigg( -\frac{68 u3}{47} \\
& + 8 a62 \bigg) \vartheta7 \bigg) \vartheta5 \bigg) e8 \bigg) + \bigg( \bigg( \bigg( \bigg( -\frac{68 u3}{47} + 8 a62 \bigg) \vartheta4 \bigg) \vartheta8 \bigg) e4 - \bigg( \bigg( \bigg( \bigg( -\frac{68 u3}{47} + 8 a62 \bigg) \vartheta7 \bigg) \vartheta4 \bigg) e9 \bigg) + \bigg( \bigg( \bigg( \bigg( \frac{120 u4}{109} \\
& + 8 a63 \bigg) \vartheta7 \bigg) \vartheta4 \bigg) e8
\end{aligned}$$

```

G > img:=DGImageSpace(x->ContractIndices(x,NJ,[[1,1],[2,2]]),GenerateTensors([DGinfo(G,
"FrameBaseVectors"),DGinfo(G,"FrameBaseVectors")]);nops(%);

```

$$\begin{aligned}
img := & \left[ -\left( \left( -\frac{68 u3}{47} + 8 a62 \right) e8 \right) - \left( \left( \frac{120 u4}{109} + 8 a63 \right) e9 \right), -\left( \left( \frac{120 u4}{109} + 8 a63 \right) e8 \right) + \left( -\frac{68 u3}{47} + 8 a62 \right) e9, \left( -\frac{68 u3}{47} \right. \right. \\
& \left. \left. + 8 a62 \right) e4 + \left( \frac{120 u4}{109} + 8 a63 \right) e5 + (4 a33 - 4 a9 - 4 a43) e6 + (4 a42 + 4 a34 + 4 a8) e7, \left( \frac{120 u4}{109} + 8 a63 \right) e4 - \left( \left( \right. \right.
\end{aligned}$$

$$\begin{aligned} & -\frac{68 u^3}{47} + 8 a62 \Big) e5 \Big) + (4 a42 + 4 a34 + 4 a8) e6 - ((4 a33 - 4 a9 - 4 a43) e7), - \Big( \Big( -\frac{68 u^3}{47} + 8 a62 \Big) e6 \Big) - \Big( \Big( \frac{120 u^4}{109} \\ & + 8 a63 \Big) e7 \Big), - \Big( \Big( \frac{120 u^4}{109} + 8 a63 \Big) e6 \Big) + \Big( -\frac{68 u^3}{47} + 8 a62 \Big) e7 \Big] \end{aligned}$$

6

(39)

The Nijenhuis tensor coefficients depend only on 10 variables. Before imposing any equations, the image has dimension 6.

**G > j1:=Query({b},"Jacobi")[2]:**

**G > eq1:={a82, a83, -6\*a82, -a82, 3\*a82, -6\*a83, -3\*a83, -a83, 3\*a83, a100-a109, 3\*a92+3\*a119}  
:sol1:=solve(eq1):**

**G > j2:=simplify(subs(sol1,j1)):**

**G > sol2:=RealDomain[solve]({op(j2[2..145]))};**

$$\begin{aligned} \text{sol2} := & \left\{ a1 = \frac{1822}{1365} a8 u9 + \frac{1822}{813} a9 u6 + 3 a30 + 3 a75, a10 = 0, a101 = 0, a102 = 0, a109 = 0, a11 = 0, a110 = 0, a111 = 0, a118 = 0, a12 \right. \\ & = \frac{451}{2439} u6 a35 + \frac{451}{4095} a4 u9 - \frac{451}{2439} u6 a72 - \frac{1230328}{3329235} u9 u6 - a57, a120 = 0, a127 = 0, a128 = 0, a129 = -\frac{253}{455} u9 a35 \\ & + \frac{253}{271} a4 u6 + \frac{271}{455} u9 a72 - \frac{18}{271} u6 a81 + \frac{1734}{73441} u6^2 + \frac{87338}{207025} u9^2 + a21 - a65, a132 = a132, a133 = a133, a19 = 0, a2 = \\ & -\frac{18}{271} a8 u6 + \frac{18}{455} a9 u9 - a39 + a66, a20 = 0, a21 = a21, a28 = -\frac{1}{3} u9 a35 + \frac{455}{813} a4 u6 + \frac{813}{455} u9 a72 + \frac{492032}{220323} u6^2 \\ & + \frac{2728}{4095} u9^2 - \frac{1984}{813} u6 a81 - 3 a65, a29 = \frac{289}{2439} u6 a35 + \frac{289}{4095} a4 u9 - \frac{18}{455} u9 a81 + \frac{3111956}{3329235} u9 u6 - \frac{451}{2439} u6 a72 - a57, \\ & a30 = a30, a33 = a33, a34 = a34, a35 = a35, a37 = \frac{2273}{813} u6 a35 + \frac{2273}{1365} a4 u9 - \frac{451}{813} u6 a72 - \frac{3776492}{1109745} u9 u6 + \frac{1822}{1365} u9 a81 \\ & - 3 a57, a38 = \frac{271}{455} u9 a35 - a4 u6 - \frac{271}{455} u9 a72 + \frac{1984}{813} u6^2 - \frac{67208}{207025} u9^2 + a65, a39 = a39, a4 = a4, a42 = a42, a43 = a43, a46 \\ & = 0, a47 = 0, a48 = -\frac{289}{455} u9 a72 + \frac{36}{271} u6 a81 + \frac{18396}{73441} u6^2 + \frac{231748}{621075} u9^2 + \frac{253}{455} u9 a35 - \frac{253}{271} a4 u6 - a21 + 2 a65, a55 = 0, \\ & a56 = 0, a57 = a57, a6 = a6, a62 = 0, a63 = 0, a64 = \frac{1822}{813} u6 a72 + \frac{1822}{1365} u9 a81 + \frac{808084}{369915} u9 u6 - 3 a57, a65 = a65, a66 = a66, a7 \\ & = a7, a72 = a72, a73 = -\frac{1984}{1365} u9 a72 + \frac{1984}{813} u6 a81 - \frac{573376}{660969} u6^2 + \frac{1984}{4095} u9^2 + 3 a65, a74 = \frac{18}{271} u6 a72 + \frac{18}{455} u9 a81 \end{aligned} \quad (40)$$



$$- \frac{433372}{369915} u_9 u_6 + a_{57}, a_{75} = a_{75}, a_8 = a_8, a_{81} = a_{81}, a_{84} = 0, a_9 = a_9, a_{91} = 0, a_{92} = 0, a_{93} = 0, u_3 = 0, u_4 = 0, u_6 = u_6, u_9 = u_9 \}$$

**G > DGbasis(DGsimpify(subs(sol2,img)));nops(%);**

$$[(4 a_{33} - 4 a_9 - 4 a_{43}) e_6 + (4 a_{42} + 4 a_{34} + 4 a_8) e_7, (4 a_{42} + 4 a_{34} + 4 a_8) e_6 - ((4 a_{33} - 4 a_9 - 4 a_{43}) e_7)]$$

2

(41)

We partially solve the Jacobi system, and see that the Nijenhuis tensor is now degenerate, of rank 2. Just as a check, we recompute by imposing the partial solution on the algebra structure from the beginning.

**g > genbrak:=subs(sol2,genbrak):**

**g > gisoten:=subs(sol2,gisoten):**

**g > streqs:=cohom\_alfromten(genbrak,gisoten);**

$$\begin{aligned} streqs := & \left[ [o1, o2] = a_4 o1 + \left( -a_{72} - \frac{2728}{1365} u_9 + a_{35} \right) o2 + a_6 o3 + a_7 o4 + a_8 o5 + a_9 o6 + \left( \frac{1822}{1365} a_8 u_9 + \frac{1822}{813} a_9 u_6 + 3 a_{30} \right. \right. \\ & + 3 a_{75} \left. \right) r1 + \left( -\frac{18}{271} a_8 u_6 + \frac{18}{455} a_9 u_9 - a_{39} + a_{66} \right) r2 + a_3 r3, [o1, o3] = \left( \frac{2273}{1365} u_9 + a_{35} \right) o3 + \left( -\frac{457}{271} u_6 - a_4 - a_{81} \right) o4 \\ & + \left( \frac{451}{2439} u_6 a_{35} + \frac{451}{4095} a_4 u_9 - \frac{451}{2439} u_6 a_{72} - \frac{1230328}{3329235} u_9 u_6 - a_{57} \right) r3, [o1, o4] = \left( -\frac{289}{813} u_6 + a_{132} + a_4 + a_{81} \right) o3 \\ & + \left( a_{133} + a_{35} + \frac{1311}{455} u_9 \right) o4 + a_{21} r3, [o1, o5] = a_{33} o3 + a_{34} o4 + a_{35} o5 + \left( \frac{248}{271} u_6 - a_4 - a_{81} \right) o6 + \left( -\frac{1}{3} u_9 a_{35} \right. \\ & + \frac{455}{813} a_4 u_6 + \frac{813}{455} u_9 a_{72} + \frac{492032}{220323} u_6^2 + \frac{2728}{4095} u_9^2 - \frac{1984}{813} u_6 a_{81} - 3 a_{65} \left. \right) r1 + \left( \frac{289}{2439} u_6 a_{35} + \frac{289}{4095} a_4 u_9 \right. \\ & - \frac{18}{455} u_9 a_{81} + \frac{3111956}{3329235} u_9 u_6 - \frac{451}{2439} u_6 a_{72} - a_{57} \left. \right) r2 + a_{30} r3, [o1, o6] = a_{42} o3 + a_{43} o4 + \left( -\frac{2728}{813} u_6 + a_4 + a_{81} \right) o5 \\ & + \left( \frac{1984}{1365} u_9 + a_{35} \right) o6 + \left( \frac{2273}{813} u_6 a_{35} + \frac{2273}{1365} a_4 u_9 - \frac{451}{813} u_6 a_{72} - \frac{3776492}{1109745} u_9 u_6 + \frac{1822}{1365} u_9 a_{81} - 3 a_{57} \right) r1 \\ & + \left( \frac{271}{455} u_9 a_{35} - a_4 u_6 - \frac{271}{455} u_9 a_{72} + \frac{1984}{813} u_6^2 - \frac{67208}{207025} u_9^2 + a_{65} \right) r2 + a_{39} r3, [o2, o3] = \left( \frac{1311}{271} u_6 - a_{132} + a_{81} \right) o3 \\ & + \left( -a_{133} + a_{72} + \frac{813}{455} u_9 \right) o4 + \left( -\frac{289}{455} u_9 a_{72} + \frac{36}{271} u_6 a_{81} + \frac{18396}{73441} u_6^2 + \frac{231748}{621075} u_9^2 + \frac{253}{455} u_9 a_{35} - \frac{253}{271} a_4 u_6 - a_{21} \right. \\ & + 2 a_{65} \left. \right) r3, [o2, o4] = \left( -a_{72} - \frac{4099}{1365} u_9 \right) o3 + \left( \frac{2273}{813} u_6 + a_{81} \right) o4 + a_{57} r3, [o2, o5] = (a_{42} + a_8) o3 + (a_{43} + a_9) o4 \\ & + \left( \frac{1984}{813} u_6 + a_{81} \right) o5 + a_{72} o6 + \left( \frac{1822}{813} u_6 a_{72} + \frac{1822}{1365} u_9 a_{81} + \frac{808084}{369915} u_9 u_6 - 3 a_{57} \right) r1 + a_{65} r2 + a_{66} r3, [o2, o6] = ( \end{aligned}$$

(42)

$$\begin{aligned}
& -a33 + a9) o3 + (-a34 - a8) o4 + \left( -a72 - \frac{1984}{1365} u9 \right) o5 + a81 o6 + \left( -\frac{1984}{1365} u9 a72 + \frac{1984}{813} u6 a81 - \frac{573376}{660969} u6^2 \right. \\
& \left. + \frac{1984}{4095} u9^2 + 3 a65 \right) r1 + \left( \frac{18}{271} u6 a72 + \frac{18}{455} u9 a81 - \frac{433372}{369915} u9 u6 + a57 \right) r2 + a75 r3, [o3, o4] = a82 r1 + a83 r2, [o3, o5] \\
& = 0, [o3, o6] = a100 r1, [o4, o5] = 0, [o4, o6] = a119 r2, [o5, o6] = a132 o3 + a133 o4 + \left( -\frac{253}{455} u9 a35 + \frac{253}{271} a4 u6 + \frac{271}{455} u9 a72 \right. \\
& \left. - \frac{18}{271} u6 a81 + \frac{1734}{73441} u6^2 + \frac{87338}{207025} u9^2 + a21 - a65 \right) r3, [r1, o1] = -o5 - \frac{2273}{1365} u9 r1 + u6 r2, [r1, o2] = -o6 - \frac{2273}{813} u6 r1 \\
& - \frac{271}{455} u9 r2, [r1, o3] = 0, [r1, o4] = 0, [r1, o5] = o3 + \frac{18}{271} u6 r3, [r1, o6] = o4 - \frac{18}{455} u9 r3, [r2, o1] = 3 o6 - \frac{455}{271} u6 r1 \\
& - \frac{289}{1365} u9 r2, [r2, o2] = -3 o5 + u9 r1 - \frac{289}{813} u6 r2, [r2, o3] = 0, [r2, o4] = 0, [r2, o5] = 3 o4 + \frac{1822}{1365} u9 r3, [r2, o6] = -3 o3 \\
& + \frac{1822}{813} u6 r3, [r3, o1] = 6 o4 - \frac{902}{1365} u9 r3, [r3, o2] = -6 o3 - \frac{902}{813} u6 r3, [r3, o3] = 0, [r3, o4] = 0, [r3, o5] = 0, [r3, o6] = 0, [r1, \\
& r2] = r3, [r1, r3] = 0, [r2, r3] = 0 \Big], [r1, r2, r3, o1, o2, o3, o4, o5, o6]
\end{aligned}$$

**G > DGsetup(LieAlgebraData(streqs,G));**

*Lie algebra: G*

(43)

**G > Jten:=evalDG(add(e||(2\*i) &t theta||(2\*i+1) - e||(2\*i+1) &t theta||(2\*i),i=2..4));**

*Jten := e4 θ5 - (e5 θ4) + e6 θ7 - (e7 θ6) + e8 θ9 - (e9 θ8)*

(44)

**G > Pf:=(x,i)->ContractIndices(mproj\_ten,convert(x,DGtensor),[[2,i]]);**

*Pf := (x, i) → DifferentialGeometry:-Tensor:-ContractIndices(mproj\_ten, convert(x, DifferentialGeometry:-Tools:-DGtensor), [[2, i]])*

(45)

**G > NJ:=Pf(Pf(Pm(TensorBrackets(Jten,Jten,"Frolicher-Nijenhuis"),1),2),3);**

$$\begin{aligned}
NJ := & \left( \left( (4 a33 - 4 a9 - 4 a43) \theta4 \right) \theta8 \right) e6 + \left( \left( (4 a42 + 4 a34 + 4 a8) \theta4 \right) \theta8 \right) e7 + \left( \left( (4 a42 + 4 a34 + 4 a8) \theta4 \right) \theta9 \right) e6 - \left( \left( (4 a33 \right. \right. \\
& \left. \left. - 4 a9 - 4 a43) \theta4 \right) \theta9 \right) e7 + \left( \left( (4 a42 + 4 a34 + 4 a8) \theta5 \right) \theta8 \right) e6 - \left( \left( (4 a33 - 4 a9 - 4 a43) \theta5 \right) \theta8 \right) e7 - \left( \left( (4 a33 \right. \right. \\
& \left. \left. - 4 a9 - 4 a43) \theta5 \right) \theta9 \right) e6 - \left( \left( (4 a42 + 4 a34 + 4 a8) \theta5 \right) \theta9 \right) e7 - \left( \left( (4 a33 - 4 a9 - 4 a43) \theta8 \right) \theta4 \right) e6 - \left( \left( (4 a42 \right. \right. \\
& \left. \left. + 4 a34 + 4 a8) \theta8 \right) \theta4 \right) e7 - \left( \left( (4 a42 + 4 a34 + 4 a8) \theta8 \right) \theta5 \right) e6 + \left( \left( (4 a33 - 4 a9 - 4 a43) \theta8 \right) \theta5 \right) e7 - \left( \left( (4 a42 \right. \right. \\
& \left. \left. + 4 a34 + 4 a8) \theta9 \right) \theta4 \right) e6 + \left( \left( (4 a33 - 4 a9 - 4 a43) \theta9 \right) \theta4 \right) e7 + \left( \left( (4 a33 - 4 a9 - 4 a43) \theta9 \right) \theta5 \right) e6 + \left( \left( (4 a42 + 4 a34 \right. \right. \\
& \left. \left. + 4 a8) \theta9 \right) \theta5 \right) e7
\end{aligned}$$

(46)

```
G > img:=DGImageSpace(x->ContractIndices(x,NJ,[[1,1],[2,2]]),GenerateTensors([DGinfo(G,
"FrameBaseVectors"),DGinfo(G,"FrameBaseVectors")]));nops(%);
img := [(4 a33 - 4 a9 - 4 a43) e6 + (4 a42 + 4 a34 + 4 a8) e7, (4 a42 + 4 a34 + 4 a8) e6 - ((4 a33 - 4 a9 - 4 a43) e7)]
```

2

(47)

This confirms that the Nijenhuis tensor for the case  $h=l_0$  is degenerate in general.

### Section 3: $h=l_1$

These representation matrices come from another worksheet. The cohomology is 4D.

```
V > MrepMat := [Matrix(9, 9, {(1, 1) = 0, (1, 2) = 0, (1, 3) = 0, (1, 4) = 0, (1, 5) = 0, (1, 6)
= 0, (1, 7) = 0, (1, 8) = 0, (1, 9) = 0, (2, 1) = 0, (2, 2) = -1, (2, 3) = 0, (2, 4) = 0, (2,
5) = 0, (2, 6) = 0, (2, 7) = 0, (2, 8) = 0, (2, 9) = 0, (3, 1) = 0, (3, 2) = 0, (3, 3) = -2,
(3, 4) = 0, (3, 5) = 0, (3, 6) = 0, (3, 7) = 0, (3, 8) = 0, (3, 9) = 0, (4, 1) = 0, (4, 2) =
0, (4, 3) = 0, (4, 4) = 1, (4, 5) = 0, (4, 6) = 0, (4, 7) = 0, (4, 8) = 0, (4, 9) = 0, (5, 1)
= 0, (5, 2) = 0, (5, 3) = 0, (5, 4) = 0, (5, 5) = 1, (5, 6) = 0, (5, 7) = 0, (5, 8) = 0, (5,
9) = 0, (6, 1) = 0, (6, 2) = 0, (6, 3) = 0, (6, 4) = 0, (6, 5) = 0, (6, 6) = -1, (6, 7) = 0,
(6, 8) = 0, (6, 9) = 0, (7, 1) = 0, (7, 2) = 0, (7, 3) = 0, (7, 4) = 0, (7, 5) = 0, (7, 6) =
0, (7, 7) = -1, (7, 8) = 0, (7, 9) = 0, (8, 1) = 0, (8, 2) = 0, (8, 3) = 0, (8, 4) = 0, (8,
5) = 0, (8, 6) = 0, (8, 7) = 0, (8, 8) = 0, (8, 9) = 0, (9, 1) = 0, (9, 2) = 0, (9, 3) = 0,
(9, 4) = 0, (9, 5) = 0, (9, 6) = 0, (9, 7) = 0, (9, 8) = 0, (9, 9) = 0}), Matrix(9, 9, {(1,
1) = 0, (1, 2) = 0, (1, 3) = 0, (1, 4) = -(6/5)*u2+(12/5)*u4, (1, 5) = (6/5)*u1-(12/5)*u3,
(1, 6) = 0, (1, 7) = 0, (1, 8) = 0, (1, 9) = 0, (2, 1) = 1, (2, 2) = 0, (2, 3) = 0, (2, 4) =
0, (2, 5) = 0, (2, 6) = 0, (2, 7) = 0, (2, 8) = 6*u2, (2, 9) = -6*u1, (3, 1) = 0, (3, 2) = 0,
(3, 3) = 0, (3, 4) = 0, (3, 5) = 0, (3, 6) = u3, (3, 7) = u4, (3, 8) = 0, (3, 9) = 0, (4, 1)
= 0, (4, 2) = 0, (4, 3) = 0, (4, 4) = 0, (4, 5) = 0, (4, 6) = 0, (4, 7) = 0, (4, 8) = 0, (4,
9) = 0, (5, 1) = 0, (5, 2) = 0, (5, 3) = 0, (5, 4) = 0, (5, 5) = 0, (5, 6) = 0, (5, 7) = 0,
(5, 8) = 0, (5, 9) = 0, (6, 1) = 0, (6, 2) = 0, (6, 3) = 0, (6, 4) = 0, (6, 5) = 0, (6, 6) =
0, (6, 7) = 0, (6, 8) = 1, (6, 9) = 0, (7, 1) = 0, (7, 2) = 0, (7, 3) = 0, (7, 4) = 0, (7, 5)
= 0, (7, 6) = 0, (7, 7) = 0, (7, 8) = 0, (7, 9) = 1, (8, 1) = 0, (8, 2) = 0, (8, 3) = 0, (8,
4) = -1, (8, 5) = 0, (8, 6) = 0, (8, 7) = 0, (8, 8) = 0, (8, 9) = 0, (9, 1) = 0, (9, 2) = 0,
(9, 3) = 0, (9, 4) = 0, (9, 5) = -1, (9, 6) = 0, (9, 7) = 0, (9, 8) = 0, (9, 9) = 0}), Matrix
(9, 9, {(1, 1) = 0, (1, 2) = 0, (1, 3) = 0, (1, 4) = 0, (1, 5) = 0, (1, 6) = 0, (1, 7) = 0,
(1, 8) = 0, (1, 9) = 0, (2, 1) = 0, (2, 2) = 0, (2, 3) = 0, (2, 4) = u1, (2, 5) = u2, (2, 6)
= 0, (2, 7) = 0, (2, 8) = 0, (2, 9) = 0, (3, 1) = 2, (3, 2) = 0, (3, 3) = 0, (3, 4) = 0, (3,
5) = 0, (3, 6) = 0, (3, 7) = 0, (3, 8) = -(12/5)*u2-(6/5)*u4, (3, 9) = (12/5)*u1+(6/5)*u3,
(4, 1) = 0, (4, 2) = 0, (4, 3) = 0, (4, 4) = 0, (4, 5) = 0, (4, 6) = 0, (4, 7) = 0, (4, 8) =
0, (4, 9) = 0, (5, 1) = 0, (5, 2) = 0, (5, 3) = 0, (5, 4) = 0, (5, 5) = 0, (5, 6) = 0, (5, 7)
```

$= 0, (5, 8) = 0, (5, 9) = 0, (6, 1) = 0, (6, 2) = 0, (6, 3) = 0, (6, 4) = 0, (6, 5) = -6, (6, 6) = 0, (6, 7) = 0, (6, 8) = 0, (6, 9) = 0, (7, 1) = 0, (7, 2) = 0, (7, 3) = 0, (7, 4) = 6, (7, 5) = 0, (7, 6) = 0, (7, 7) = 0, (7, 8) = 0, (7, 9) = 0, (8, 1) = 0, (8, 2) = 0, (8, 3) = 0, (8, 4) = 0, (8, 5) = 0, (8, 6) = 0, (8, 7) = 0, (8, 8) = 0, (8, 9) = 0, (9, 1) = 0, (9, 2) = 0, (9, 3) = 0, (9, 4) = 0, (9, 5) = 0, (9, 6) = 0, (9, 7) = 0, (9, 8) = 0, (9, 9) = 0\}]];$

$$MrepMat := \left[ \begin{bmatrix} 0 & 0 & 0 & 0 & 0 & 0 & 0 & 0 & 0 \\ 0 & -1 & 0 & 0 & 0 & 0 & 0 & 0 & 0 \\ 0 & 0 & -2 & 0 & 0 & 0 & 0 & 0 & 0 \\ 0 & 0 & 0 & 1 & 0 & 0 & 0 & 0 & 0 \\ 0 & 0 & 0 & 0 & 1 & 0 & 0 & 0 & 0 \\ 0 & 0 & 0 & 0 & 0 & -1 & 0 & 0 & 0 \\ 0 & 0 & 0 & 0 & 0 & 0 & -1 & 0 & 0 \\ 0 & 0 & 0 & 0 & 0 & 0 & 0 & 0 & 0 \\ 0 & 0 & 0 & 0 & 0 & 0 & 0 & 0 & 0 \end{bmatrix}, \begin{bmatrix} 0 & 0 & 0 & -\frac{6}{5}u_2 + \frac{12}{5}u_4 & \frac{6}{5}u_1 - \frac{12}{5}u_3 & 0 & 0 & 0 & 0 \\ 1 & 0 & 0 & 0 & 0 & 0 & 0 & 6u_2 & -6u_1 \\ 0 & 0 & 0 & 0 & 0 & u_3 & u_4 & 0 & 0 \\ 0 & 0 & 0 & 0 & 0 & 0 & 0 & 0 & 0 \\ 0 & 0 & 0 & 0 & 0 & 0 & 0 & 0 & 0 \\ 0 & 0 & 0 & 0 & 0 & 0 & 0 & 0 & 0 \\ 0 & 0 & 0 & 0 & 0 & 0 & 0 & 1 & 0 \\ 0 & 0 & 0 & 0 & 0 & 0 & 0 & 0 & 1 \\ 0 & 0 & 0 & -1 & 0 & 0 & 0 & 0 & 0 \\ 0 & 0 & 0 & 0 & -1 & 0 & 0 & 0 & 0 \end{bmatrix} \right],$$

(48)

$$\left[ \begin{bmatrix} 0 & 0 & 0 & 0 & 0 & 0 & 0 & 0 \\ 0 & 0 & 0 & u_1 & u_2 & 0 & 0 & 0 \\ 2 & 0 & 0 & 0 & 0 & 0 & 0 & -\frac{12}{5}u_2 - \frac{6}{5}u_4 \\ 0 & 0 & 0 & 0 & 0 & 0 & 0 & 0 \\ 0 & 0 & 0 & 0 & 0 & 0 & 0 & 0 \\ 0 & 0 & 0 & 0 & -6 & 0 & 0 & 0 \\ 0 & 0 & 0 & 6 & 0 & 0 & 0 & 0 \\ 0 & 0 & 0 & 0 & 0 & 0 & 0 & 0 \\ 0 & 0 & 0 & 0 & 0 & 0 & 0 & 0 \end{bmatrix}, \begin{bmatrix} 0 \\ 0 \\ \frac{12}{5}u_1 + \frac{6}{5}u_3 \\ 0 \\ 0 \\ 0 \\ 0 \\ 0 \\ 0 \\ 0 \end{bmatrix} \right]$$

V80 > HData:=simplify(LieAlgebraData(MrepMat,h));DGsetup(HData);  
HData := [[e1, e2] = -e2, [e1, e3] = -2 e3]

`V > DGsetup([seq(v | i, i=1..dimM)], m);` Lie algebra: h (49)

`m > DGsetup([seq(w | i, i=1..9)], g);` frame name: m (50)

`g > rep:=Representation(h, g, MrepMat);` frame name: g (51)

`V > Mrep:=TensorProductOfRepresentations(rep, [seq(dw | i, i=4..9)], m);`

$$Mrep := \left[ \begin{array}{c} e1, \\ \begin{bmatrix} -1 & 0 & 0 & 0 & 0 & 0 \\ 0 & -1 & 0 & 0 & 0 & 0 \\ 0 & 0 & 1 & 0 & 0 & 0 \\ 0 & 0 & 0 & 1 & 0 & 0 \\ 0 & 0 & 0 & 0 & 0 & 0 \\ 0 & 0 & 0 & 0 & 0 & 0 \end{bmatrix} \end{array} \right], \left[ \begin{array}{c} e2, \\ \begin{bmatrix} 0 & 0 & 0 & 0 & 1 & 0 \\ 0 & 0 & 0 & 0 & 0 & 1 \\ 0 & 0 & 0 & 0 & 0 & 0 \\ 0 & 0 & 0 & 0 & 0 & 0 \\ 0 & 0 & -1 & 0 & 0 & 0 \\ 0 & 0 & 0 & -1 & 0 & 0 \end{bmatrix} \end{array} \right], \left[ \begin{array}{c} e3, \\ \begin{bmatrix} 0 & 0 & 0 & -6 & 0 & 0 \\ 0 & 0 & 6 & 0 & 0 & 0 \\ 0 & 0 & 0 & 0 & 0 & 0 \\ 0 & 0 & 0 & 0 & 0 & 0 \\ 0 & 0 & 0 & 0 & 0 & 0 \\ 0 & 0 & 0 & 0 & 0 & 0 \end{bmatrix} \end{array} \right]$$
(52)

`G > ChangeFrame(g);` h (53)

`g > L2M:=GenerateForms(DGinfo(g, "FrameBaseForms")[4..9], 2);`  
 $L2M := [dw4 \wedge dw5, dw4 \wedge dw6, dw4 \wedge dw7, dw4 \wedge dw8, dw4 \wedge dw9, dw5 \wedge dw6, dw5 \wedge dw7, dw5 \wedge dw8, dw5 \wedge dw9, dw6 \wedge dw7,$  (54)  
 $dw6 \wedge dw8, dw6 \wedge dw9, dw7 \wedge dw8, dw7 \wedge dw9, dw8 \wedge dw9]$

`g > brakspace:=GenerateTensors([L2M, DGinfo(g, "FrameBaseVectors")]):`

`g > genbrak:=evalDG(add(a | i*brakspace[i], i=1..nops(brakspace))):`

`g > gisoten:=map(x->convert(x, DGtensor, [{"con_bas", "cov_bas"}, []]), MrepMat);` (55)

$$gisoten := \left[ - (D_{w2} dw2) - ((2 D_{w3}) dw3) + D_{w4} dw4 + D_{w5} dw5 - (D_{w6} dw6) - (D_{w7} dw7), - \left( \left( \frac{6 u2}{5} - \frac{12 u4}{5} \right) D_{w1} \right) dw4 \right) + \left( \left( \frac{6 u1}{5} - \frac{12 u3}{5} \right) D_{w1} \right) dw5 + D_{w2} dw1 + (6 u2 D_{w2}) dw8 - ((6 u1 D_{w2}) dw9) \right. \\ \left. + (u3 D_{w3}) dw6 + (u4 D_{w3}) dw7 + D_{w6} dw8 + D_{w7} dw9 - (D_{w8} dw4) - (D_{w9} dw5), (u1 D_{w2}) dw4 + (u2 D_{w2}) dw5 \right. \\ \left. + (2 D_{w3}) dw1 - \left( \left( \left( \frac{12 u2}{5} + \frac{6 u4}{5} \right) D_{w3} \right) dw8 \right) + \left( \left( \frac{12 u1}{5} + \frac{6 u3}{5} \right) D_{w3} \right) dw9 - ((6 D_{w6}) dw5) + (6 D_{w7}) dw4 \right]$$

`g > streqs:=cohom_algfromten(genbrak, gisoten);`

$$\begin{aligned}
\text{streqs} := & \left[ [o1, o2] = a1\ r1 + a2\ r2 + a3\ r3 + a4\ o1 + a5\ o2 + a6\ o3 + a7\ o4 + a8\ o5 + a9\ o6, [o1, o3] = a10\ r1 + a11\ r2 + a12\ r3 + a13\ o1 \right. \\
& + a14\ o2 + a15\ o3 + a16\ o4 + a17\ o5 + a18\ o6, [o1, o4] = a19\ r1 + a20\ r2 + a21\ r3 + a22\ o1 + a23\ o2 + a24\ o3 + a25\ o4 + a26\ o5 \\
& + a27\ o6, [o1, o5] = a28\ r1 + a29\ r2 + a30\ r3 + a31\ o1 + a32\ o2 + a33\ o3 + a34\ o4 + a35\ o5 + a36\ o6, [o1, o6] = a37\ r1 + a38\ r2 \\
& + a39\ r3 + a40\ o1 + a41\ o2 + a42\ o3 + a43\ o4 + a44\ o5 + a45\ o6, [o2, o3] = a46\ r1 + a47\ r2 + a48\ r3 + a49\ o1 + a50\ o2 + a51\ o3 \\
& + a52\ o4 + a53\ o5 + a54\ o6, [o2, o4] = a55\ r1 + a56\ r2 + a57\ r3 + a58\ o1 + a59\ o2 + a60\ o3 + a61\ o4 + a62\ o5 + a63\ o6, [o2, o5] \\
& = a64\ r1 + a65\ r2 + a66\ r3 + a67\ o1 + a68\ o2 + a69\ o3 + a70\ o4 + a71\ o5 + a72\ o6, [o2, o6] = a73\ r1 + a74\ r2 + a75\ r3 + a76\ o1 \\
& + a77\ o2 + a78\ o3 + a79\ o4 + a80\ o5 + a81\ o6, [o3, o4] = a82\ r1 + a83\ r2 + a84\ r3 + a85\ o1 + a86\ o2 + a87\ o3 + a88\ o4 + a89\ o5 \\
& + a90\ o6, [o3, o5] = a91\ r1 + a92\ r2 + a93\ r3 + a94\ o1 + a95\ o2 + a96\ o3 + a97\ o4 + a98\ o5 + a99\ o6, [o3, o6] = a100\ r1 + a101\ r2 \\
& + a102\ r3 + a103\ o1 + a104\ o2 + a105\ o3 + a106\ o4 + a107\ o5 + a108\ o6, [o4, o5] = a109\ r1 + a110\ r2 + a111\ r3 + a112\ o1 \\
& + a113\ o2 + a114\ o3 + a115\ o4 + a116\ o5 + a117\ o6, [o4, o6] = a118\ r1 + a119\ r2 + a120\ r3 + a121\ o1 + a122\ o2 + a123\ o3 \\
& + a124\ o4 + a125\ o5 + a126\ o6, [o5, o6] = a127\ r1 + a128\ r2 + a129\ r3 + a130\ o1 + a131\ o2 + a132\ o3 + a133\ o4 + a134\ o5 \\
& + a135\ o6, [r1, o1] = o1, [r1, o2] = o2, [r1, o3] = -o3, [r1, o4] = -o4, [r1, o5] = 0, [r1, o6] = 0, [r2, o1] = -o5 + \left( -\frac{6}{5} u2 \right. \\
& + \left. \frac{12}{5} u4 \right) r1, [r2, o2] = -o6 + \left( \frac{6}{5} u1 - \frac{12}{5} u3 \right) r1, [r2, o3] = u3\ r3, [r2, o4] = u4\ r3, [r2, o5] = 6\ r2\ u2 + o3, [r2, o6] = -6\ r2\ u1 \\
& + o4, [r3, o1] = r2\ u1 + 6\ o4, [r3, o2] = r2\ u2 - 6\ o3, [r3, o3] = 0, [r3, o4] = 0, [r3, o5] = \left( -\frac{12}{5} u2 - \frac{6}{5} u4 \right) r3, [r3, o6] = \left( \frac{12}{5} u1 \right. \\
& + \left. \frac{6}{5} u3 \right) r3, [r1, r2] = -r2, [r1, r3] = -2\ r3, [r2, r3] = 0 \Big], [r1, r2, r3, o1, o2, o3, o4, o5, o6]
\end{aligned}$$

**g > DGsetup(LieAlgebraData(streqs,G));**

*Lie algebra: G*

(57)

```
g > Jac:=(x,y,z)->evalDG(LieBracket(LieBracket(x,y),z)+LieBracket(LieBracket(z,x),y)+LieBracket(LieBracket(y,z),x));
```

(58)

```
Jac := (x, y, z) → DifferentialGeometry:-evalDG(DifferentialGeometry:-LieBracket(DifferentialGeometry:-LieBracket(x, y), z) + DifferentialGeometry:-LieBracket(DifferentialGeometry:-LieBracket(z, x), y) + DifferentialGeometry:-LieBracket(DifferentialGeometry:-LieBracket(y, z), x))
```

```
g > mproj_ten:=evalDG(add(theta||i &t e||i,i=4..9));
```

(59)

$mproj\_ten := \theta_4 e_4 + \theta_5 e_5 + \theta_6 e_6 + \theta_7 e_7 + \theta_8 e_8 + \theta_9 e_9$

```
g > Pm:=(x,i)->ContractIndices(mproj_ten,convert(x,DGtensor),[[1,i]]);
```

(60)

$Pm := (x, i) \rightarrow DifferentialGeometry:-Tensor:-ContractIndices(mproj\_ten, convert(x, DifferentialGeometry:-Tools:-DGtensor), [[1, i]])$

```
g > {seq(seq(seq(op(DGinfo(evalDG(convert(Jac(e||i,e||j,e||k),DGtensor) &minus Pm(Jac(e||i,e||j,e||k),1)), "CoefficientSet")), i=1..3), j=1..3), k=4..9)};
```

(61)

$\{0\}$

```
G > {seq(seq(seq(op(DGinfo(Pm(Jac(e||i,e||j,e||k),1), "CoefficientSet")), i=1..3), j=1..3), k=4..9)};
```

(62)

$\{0\}$

```
G > dd_eq:={seq(seq(seq(op(DGinfo(Pm(Jac(e||i,e||j,e||k),1), "CoefficientSet")), i=1..3), j=4..9), k=4..9)};
```

```
G > dd_sol:=solve(dd_eq);
```

(63)

$dd\_sol := \left\{ a_{103} = 0, a_{104} = 0, a_{105} = a_{105}, a_{106} = \frac{365}{442} a_{115} - \frac{77}{442} a_{68}, a_{107} = 0, a_{108} = 0, a_{112} = 0, a_{113} = 0, a_{114} = \frac{365}{442} a_{105} \right.$

$\left. - \frac{77}{442} a_{40}, a_{115} = a_{115}, a_{116} = 0, a_{117} = 0, a_{121} = 0, a_{122} = 0, a_{123} = -\frac{147}{221} a_{115} - \frac{368}{221} a_{68}, a_{124} = -\frac{79}{442} a_{105} + \frac{363}{442} a_{40}, \right.$

$a_{125} = 0, a_{126} = 0, a_{13} = 0, a_{130} = 0, a_{131} = 0, a_{132} = 0, a_{133} = 0, a_{134} = \frac{1}{2} a_{105} + \frac{1}{2} a_{40}, a_{135} = -\frac{1}{2} a_{68} - \frac{1}{2} a_{115}, a_{14} = 0, a_{15}$

$= 0, a_{16} = 0, a_{17} = -\frac{373}{442} a_{115} + \frac{69}{442} a_{68}, a_{18} = \frac{369}{442} a_{105} - \frac{73}{442} a_{40}, a_{22} = 0, a_{23} = 0, a_{24} = 0, a_{25} = 0, a_{26} = \frac{365}{442} a_{105}$

$\left. - \frac{77}{442} a_{40}, a_{27} = -\frac{957}{442} a_{68} - \frac{515}{442} a_{115}, a_{31} = \frac{517}{442} a_{115} + \frac{75}{442} a_{68}, a_{32} = -\frac{369}{442} a_{105} + \frac{73}{442} a_{40}, a_{33} = 0, a_{34} = 0, a_{35} = 0, \right.$

$a_{36} = 0, a_4 = 0, a_{40} = a_{40}, a_{41} = \frac{147}{221} a_{115} + \frac{368}{221} a_{68}, a_{42} = 0, a_{43} = 0, a_{44} = 0, a_{45} = 0, a_{49} = 0, a_5 = 0, a_{50} = 0, a_{51} = 0, a_{52} = 0, a_{53}$

$\left. = -\frac{515}{442} a_{105} - \frac{957}{442} a_{40}, a_{54} = \frac{365}{442} a_{115} - \frac{77}{442} a_{68}, a_{58} = 0, a_{59} = 0, a_6 = 0, a_{60} = 0, a_{61} = 0, a_{62} = \frac{369}{442} a_{115} - \frac{73}{442} a_{68}, a_{63} \right.$

$$\begin{aligned}
&= -\frac{373}{442} a_{105} + \frac{69}{442} a_{40}, a_{67} = \frac{147}{221} a_{105} + \frac{368}{221} a_{40}, a_{68} = a_{68}, a_{69} = 0, a_7 = 0, a_{70} = 0, a_{71} = 0, a_{72} = 0, a_{76} = -\frac{369}{442} a_{115} \\
&+ \frac{73}{442} a_{68}, a_{77} = \frac{517}{442} a_{105} + \frac{75}{442} a_{40}, a_{78} = 0, a_{79} = 0, a_8 = 0, a_{80} = 0, a_{81} = 0, a_{85} = 0, a_{86} = 0, a_{87} = 0, a_{88} = 0, a_{89} = 0, a_9 = 0, \\
&a_{90} = 0, a_{94} = 0, a_{95} = 0, a_{96} = -\frac{79}{442} a_{115} + \frac{363}{442} a_{68}, a_{97} = -\frac{147}{221} a_{105} - \frac{368}{221} a_{40}, a_{98} = 0, a_{99} = 0, u_1 = \frac{12}{221} a_{105} + \frac{12}{221} a_{40}, \\
&u_2 = -\frac{12}{221} a_{115} - \frac{12}{221} a_{68}, u_3 = -\frac{1}{4} a_{105} - \frac{1}{4} a_{40}, u_4 = \frac{1}{4} a_{115} + \frac{1}{4} a_{68} \}
\end{aligned}$$

```

g > genbrak2:=subs(dd_sol,genbrak):
g > gisoten2:=subs(dd_sol,gisoten):
g > streqs2:=cohom_algfromten(genbrak2,gisoten2):
g > DGsetup(LieAlgebraData(streqs2,G));

```

*Lie algebra: G*

(64)

Up to this point, the procedure is the same as in Section 1. Now we deviate by attacking the full Jacobi system instead of the system  $[Q\phi]=0$ .

```

G > jaceq:=Query({a},"Jacobi")[2]:
G > jacgrob:=Groebner[Basis](%, 'terat');

```

```

jacgrob := [a127, a128, a129, a56, a11, a101 - a110, a47, 221 a55 - 146 a10 + 98 a92, a100, a109, a102, a111, a38, a65, a12, a57, a20,
367 a46 - 98 a110, 367 a19 - 98 a110, 21658 a119 + 27525 a10 + 14308 a92, a83, a28, a37, a93, a120, a29, a74, a21, a48, 588 a84
+ 367 a10 - 98 a92, a73, a64, a91, a118, a39, a66, a1, a2, a30, a75, a82, a3, -431592 a105^2 - 691488 a105 a40 + 259896 a115^2
+ 10578065 a10 - 7890862 a92, 2202 a105 a115 + 1101 a105 a68 + 1101 a115 a40 - 113815 a110, 171696 a105^2 + 431592 a105 a40
+ 259896 a115 a68 - 12998015 a10 + 4728794 a92, 147 a105^2 + 294 a105 a40 + 147 a40^2 - 16133 a10 + 10829 a92, -367 a105 a115
+ 367 a40 a68 + 21658 a110, -26791 a10 a115 + 14406 a105 a110 + 25235 a110 a40 + 17983 a115 a92, 361169471 a10 a105
- 195279966 a105 a92 - 137469514 a110 a115 + 38632622 a40 a92, 107898 a10 a105 + 189005 a10 a40 - 21658 a110 a115,
29400 a105^2 - 57232 a105 a40 + 86632 a68^2 - 9252493 a10 - 522242 a92, -81107 a10 a105 + 28812 a110 a115 + 50470 a110 a68,
-16306177 a10 a115 + 4623983 a105 a110 + 1582504 a115 a92 + 1852249 a68 a92, -73654331 a10 a115 + 13797365 a10 a68
+ 20726706 a105 a110 + 2625518 a115 a92, 9832297 a10^2 - 6599761 a10 a92 - 1061242 a110^2, -16310069903322 a10 a105^2
+ 9013821578580 a105^2 a92 + 4658544056712 a105 a110 a115 - 26984100017195 a10 a92 + 90442911629525 a110^2
+ 18112615080035 a92^2, 548179092 a10 a105 a115 - 114874032 a105^2 a110 - 31506216 a105 a115 a92 - 8351917225 a10 a110
+ 268954630 a110 a92, -29766269 a10 a105 a92 + 163061770 a10 a110 a115 - 46239830 a105 a110^2 - 5251036 a110 a115 a92,

```

(65)



$$\begin{aligned}
& 12640931485 a_{10} a_{105} a_{110} + 1435515362 a_{10} a_{115} a_{92} - 7606701102 a_{105} a_{110} a_{92} - 4811432990 a_{110}^2 a_{115} \\
& - 963565106 a_{115} a_{92}^2, 4915899325350 a_{10} a_{105}^2 a_{92} + 3868067124012 a_{105}^2 a_{110}^2 + 2555374661112 a_{105}^2 a_{92}^2 \\
& - 796209432655325 a_{10} a_{110}^2 - 7649861364098 a_{10} a_{92}^2 + 51280252807420 a_{110}^2 a_{92} + 5134838449874 a_{92}^3, \\
& 2994214698370861758 a_{10} a_{105}^2 a_{110} - 1426999709774222220 a_{105}^2 a_{110} a_{92} + 627454640454482568 a_{105} a_{115} a_{92}^2 \\
& + 4271917583165871005 a_{10} a_{110} a_{92} - 66523592586772700925 a_{110}^3 - 12820814070840259127 a_{110} a_{92}^2, \\
& - 12706996081675 a_{10} a_{105} a_{110}^2 - 263417068927 a_{10} a_{105} a_{92}^2 + 7237255472720 a_{105} a_{110}^2 a_{92} + 4836578714450 a_{110}^3 a_{115} \\
& + 922131806442 a_{110} a_{115} a_{92}^2, -1804135052403450 a_{10} a_{105}^2 a_{110}^2 + 1901338768396704 a_{105}^2 a_{110}^2 a_{92} \\
& + 1419580634512404 a_{105}^2 a_{92}^3 - 216960977107354400 a_{10} a_{110}^2 a_{92} - 4249707572999291 a_{10} a_{92}^3 + 40083146096004375 a_{110}^4 \\
& + 28872698256695440 a_{110}^2 a_{92}^2 + 2852543439410483 a_{92}^4]
\end{aligned}$$

**G > jacgroblinsol:=solve(jacgrob[1..42]);**

$$\begin{aligned}
& \text{jacgroblinsol} := \left\{ a_1 = 0, a_{10} = a_{10}, a_{100} = 0, a_{101} = a_{110}, a_{102} = 0, a_{109} = 0, a_{11} = 0, a_{110} = a_{110}, a_{111} = 0, a_{118} = 0, a_{119} = -\frac{146}{221} a_{92} \right. \\
& - \frac{27525}{21658} a_{10}, a_{12} = 0, a_{120} = 0, a_{127} = 0, a_{128} = 0, a_{129} = 0, a_{19} = \frac{98}{367} a_{110}, a_2 = 0, a_{20} = 0, a_{21} = 0, a_{28} = 0, a_{29} = 0, a_3 = 0, a_{30} \\
& = 0, a_{37} = 0, a_{38} = 0, a_{39} = 0, a_{46} = \frac{98}{367} a_{110}, a_{47} = 0, a_{48} = 0, a_{55} = -\frac{98}{221} a_{92} + \frac{146}{221} a_{10}, a_{56} = 0, a_{57} = 0, a_{64} = 0, a_{65} = 0, a_{66} \\
& = 0, a_{73} = 0, a_{74} = 0, a_{75} = 0, a_{82} = 0, a_{83} = 0, a_{84} = \frac{1}{6} a_{92} - \frac{367}{588} a_{10}, a_{91} = 0, a_{92} = a_{92}, a_{93} = 0 \left. \right\}
\end{aligned} \tag{66}$$

We solve the linear equations first.

**G > nolin\_jacgrob:={op(subs(jacgroblinsol,jacgrob))};**

$$\begin{aligned}
& \text{nolin\_jacgrob} := \{0, 9832297 a_{10}^2 - 6599761 a_{10} a_{92} - 1061242 a_{110}^2, 107898 a_{10} a_{105} + 189005 a_{10} a_{40} - 21658 a_{110} a_{115}, \\
& - 81107 a_{10} a_{105} + 28812 a_{110} a_{115} + 50470 a_{110} a_{68}, -367 a_{105} a_{115} + 367 a_{40} a_{68} + 21658 a_{110}, -29766269 a_{10} a_{105} a_{92} \\
& + 163061770 a_{10} a_{110} a_{115} - 46239830 a_{105} a_{110}^2 - 5251036 a_{110} a_{115} a_{92}, 2202 a_{105} a_{115} + 1101 a_{105} a_{68} + 1101 a_{115} a_{40} \\
& - 113815 a_{110}, -26791 a_{10} a_{115} + 14406 a_{105} a_{110} + 25235 a_{110} a_{40} + 17983 a_{115} a_{92}, 361169471 a_{10} a_{105} \\
& - 195279966 a_{105} a_{92} - 137469514 a_{110} a_{115} + 38632622 a_{40} a_{92}, -16306177 a_{10} a_{115} + 4623983 a_{105} a_{110} + 1582504 a_{115} a_{92} \\
& + 1852249 a_{68} a_{92}, -73654331 a_{10} a_{115} + 13797365 a_{10} a_{68} + 20726706 a_{105} a_{110} + 2625518 a_{115} a_{92}, 147 a_{105}^2 + 294 a_{105} a_{40} \\
& + 147 a_{40}^2 - 16133 a_{10} + 10829 a_{92}, 548179092 a_{10} a_{105} a_{115} - 114874032 a_{105}^2 a_{110} - 31506216 a_{105} a_{115} a_{92} \\
& - 8351917225 a_{10} a_{110} + 268954630 a_{110} a_{92}, 12640931485 a_{10} a_{105} a_{110} + 1435515362 a_{10} a_{115} a_{92}
\end{aligned} \tag{67}$$

$-7606701102 a_{105} a_{110} a_{92} - 4811432990 a_{110}^2 a_{115} - 963565106 a_{115} a_{92}^2, -12706996081675 a_{10} a_{105} a_{110}^2$   
 $-263417068927 a_{10} a_{105} a_{92}^2 + 7237255472720 a_{105} a_{110}^2 a_{92} + 4836578714450 a_{110}^3 a_{115} + 922131806442 a_{110} a_{115} a_{92}^2,$   
 $-431592 a_{105}^2 - 691488 a_{105} a_{40} + 259896 a_{115}^2 + 10578065 a_{10} - 7890862 a_{92}, 29400 a_{105}^2 - 57232 a_{105} a_{40} + 86632 a_{68}^2$   
 $-9252493 a_{10} - 522242 a_{92}, 171696 a_{105}^2 + 431592 a_{105} a_{40} + 259896 a_{115} a_{68} - 12998015 a_{10} + 4728794 a_{92},$   
 $-16310069903322 a_{10} a_{105}^2 + 9013821578580 a_{105}^2 a_{92} + 4658544056712 a_{105} a_{110} a_{115} - 26984100017195 a_{10} a_{92}$   
 $+ 90442911629525 a_{110}^2 + 18112615080035 a_{92}^2, 2994214698370861758 a_{10} a_{105}^2 a_{110} - 1426999709774222220 a_{105}^2 a_{110} a_{92}$   
 $+ 627454640454482568 a_{105} a_{115} a_{92}^2 + 4271917583165871005 a_{10} a_{110} a_{92} - 66523592586772700925 a_{110}^3$   
 $-12820814070840259127 a_{110} a_{92}^2, 4915899325350 a_{10} a_{105}^2 a_{92} + 3868067124012 a_{105}^2 a_{110}^2 + 2555374661112 a_{105}^2 a_{92}^2$   
 $-796209432655325 a_{10} a_{110}^2 - 7649861364098 a_{10} a_{92}^2 + 51280252807420 a_{110}^2 a_{92} + 5134838449874 a_{92}^3,$   
 $-1804135052403450 a_{10} a_{105}^2 a_{110}^2 + 1901338768396704 a_{105}^2 a_{110}^2 a_{92} + 1419580634512404 a_{105}^2 a_{92}^3$   
 $-216960977107354400 a_{10} a_{110}^2 a_{92} - 4249707572999291 a_{10} a_{92}^3 + 40083146096004375 a_{110}^4 + 28872698256695440 a_{110}^2 a_{92}^2$   
 $+ 2852543439410483 a_{92}^4\}$

**G > sol\_nolin\_jacgrob:=Groebner[Basis](nolin\_jacgrob,'adsgr');**

$sol\_nolin\_jacgrob := [135423 a_{105} a_{92} + 6359 a_{110} a_{115} - 155855 a_{110} a_{68} - 26791 a_{40} a_{92}, 59941 a_{105} a_{110} + 222155 a_{110} a_{40}$   
 $+ 135423 a_{115} a_{92} - 26791 a_{68} a_{92}, 229411333 a_{10} a_{68} + 9837373 a_{110} a_{40} - 69201153 a_{115} a_{92} - 140298228 a_{68} a_{92},$   
 $-116032 a_{115} a_{68} + 86632 a_{40}^2 - 29400 a_{68}^2 - 564693 a_{10} + 4447926 a_{92}, 1101 a_{105} a_{68} + 1101 a_{115} a_{40} + 2202 a_{40} a_{68}$   
 $+ 16133 a_{110}, 515759413 a_{10} a_{40} - 968816142 a_{105} a_{92} + 1298202178 a_{110} a_{68} + 191662814 a_{40} a_{92}, 86632 a_{105} a_{40}$   
 $+ 29400 a_{115} a_{68} - 57232 a_{68}^2 + 4642143 a_{10} + 879942 a_{92}, 294 a_{115}^2 + 588 a_{115} a_{68} + 294 a_{68}^2 - 48841 a_{10}, 3142621 a_{10} a_{115}$   
 $+ 3302845 a_{110} a_{40} + 1708385 a_{115} a_{92} - 755286 a_{68} a_{92}, 367 a_{105} a_{115} - 367 a_{40} a_{68} - 21658 a_{110}, 9832297 a_{10}^2$   
 $- 6599761 a_{10} a_{92} - 1061242 a_{110}^2, 515759413 a_{10} a_{105} + 3901807476 a_{105} a_{92} - 4811432990 a_{110} a_{68} - 771902292 a_{40} a_{92},$   
 $259896 a_{105}^2 + 171696 a_{115} a_{68} + 431592 a_{68}^2 - 54681923 a_{10} + 522242 a_{92}, -30595988472 a_{105} a_{68} a_{92}$   
 $+ 35005132344 a_{110} a_{68}^2 + 4409143872 a_{40} a_{68} a_{92} - 8936550701 a_{10} a_{110} - 70927459330 a_{110} a_{92},$   
 $1835269081464 a_{110} a_{40} a_{68} + 853993988232 a_{115} a_{68} a_{92} - 981275093232 a_{68}^2 a_{92} + 94053879173943 a_{10} a_{92}$   
 $+ 1179323949986 a_{110}^2]$

**G > branch:=RealDomain[solve](sol\_nolin\_jacgrob);**

(68)

(69)

$$\begin{aligned}
branch := & \left\{ a10 = \frac{392}{45387} a68^2, a105 = 0, a110 = 0, a115 = \frac{73}{369} a68, a40 = 0, a68 = a68, a92 = \frac{584}{45387} a68^2 \right\}, \left\{ a10 = 0, a105 = \frac{73}{369} a40, \right. \\
& a110 = 0, a115 = 0, a40 = a40, a68 = 0, a92 = -\frac{884}{45387} a40^2 \left. \right\}, \left\{ a10 = \frac{294}{5329} a68^2, a105 = \frac{221}{3} \text{RootOf}(218489 \_Z^2 - 515, \text{label} \right. \\
& = \_L114) a68, a110 = -\frac{367}{73} \text{RootOf}(218489 \_Z^2 - 515, \text{label} = \_L114) a68^2, a115 = -\frac{294}{73} a68, a40 = 0, a68 = a68, a92 = \\
& -\frac{59941}{655467} a68^2 \left. \right\}, \left\{ a10 = \frac{50470}{655467} a40^2, a105 = -\frac{294}{73} a40, a110 = -\frac{367}{73} \text{RootOf}(218489 \_Z^2 - 515, \text{label} = \_L116) a40^2, a115 \right. \\
& = \frac{221}{3} \text{RootOf}(218489 \_Z^2 - 515, \text{label} = \_L116) a40, a40 = a40, a68 = 0, a92 = -\frac{6359}{655467} a40^2 \left. \right\}, \left\{ a10 \right. \\
& = \frac{294}{48841} \text{RootOf}(1966401 \_Z^3 + 15449939 \_Z^2 a68 + (-25153115 a40^2 + 28761432 a68^2) \_Z - 46740837 a40^2 a68 - 6309828 a68^3)^2 \\
& + \frac{588}{48841} \text{RootOf}(1966401 \_Z^3 + 15449939 \_Z^2 a68 + (-25153115 a40^2 + 28761432 a68^2) \_Z - 46740837 a40^2 a68 \\
& - 6309828 a68^3) a68 + \frac{294}{48841} a68^2, a105 = -\frac{1}{81549} \frac{1}{a40} (26937 \text{RootOf}(1966401 \_Z^3 + 15449939 \_Z^2 a68 + (-25153115 a40^2 + 28761432 a68^2) \_Z - 46740837 a40^2 a68 - 6309828 a68^3)^2 \\
& + 103157 \text{RootOf}(1966401 \_Z^3 + 15449939 \_Z^2 a68 + (-25153115 a40^2 + 28761432 a68^2) \_Z - 46740837 a40^2 a68 - 6309828 a68^3) a68 - 16133 a40^2 - 21462 a68^2), a110 \\
& = \frac{367}{438543339} \frac{1}{a40} (26937 a68 \text{RootOf}(1966401 \_Z^3 + 15449939 \_Z^2 a68 + (-25153115 a40^2 + 28761432 a68^2) \_Z - 46740837 a40^2 a68 - 6309828 a68^3)^2 \\
& - 81549 \text{RootOf}(1966401 \_Z^3 + 15449939 \_Z^2 a68 + (-25153115 a40^2 + 28761432 a68^2) \_Z - 46740837 a40^2 a68 - 6309828 a68^3) a40^2 + 103157 \text{RootOf}(1966401 \_Z^3 + 15449939 \_Z^2 a68 + (-25153115 a40^2 + 28761432 a68^2) \_Z - 46740837 a40^2 a68 - 6309828 a68^3) a68^2 - 179231 a40^2 a68 - 21462 a68^3), a115 = \text{RootOf}(1966401 \_Z^3
\end{aligned}$$

$$\begin{aligned}
& + 15449939 \_Z^2 a68 + (-25153115 a40^2 + 28761432 a68^2) \_Z - 46740837 a40^2 a68 - 6309828 a68^3), a40 = a40, a68 = a68, a92 \\
& = \frac{4591}{6007443} \text{RootOf}(1966401 \_Z^3 + 15449939 \_Z^2 a68 + (-25153115 a40^2 + 28761432 a68^2) \_Z - 46740837 a40^2 a68 \\
& - 6309828 a68^3)^2 + \frac{61215902}{2216746467} \text{RootOf}(1966401 \_Z^3 + 15449939 \_Z^2 a68 + (-25153115 a40^2 + 28761432 a68^2) \_Z \\
& - 46740837 a40^2 a68 - 6309828 a68^3) a68 - \frac{884}{45387} a40^2 + \frac{5448793}{738915489} a68^2 \}
\end{aligned}$$

We obtain 5 families of solutions to the full Jacobi system. These families actually define Lie algebras. Now we must verify that they are all isomorphic.

**G > branch[1];**

$$\left\{ a10 = \frac{392}{45387} a68^2, a105 = 0, a110 = 0, a115 = \frac{73}{369} a68, a40 = 0, a68 = a68, a92 = \frac{584}{45387} a68^2 \right\} \quad (70)$$

**G > branch[2];**

$$\left\{ a10 = 0, a105 = \frac{73}{369} a40, a110 = 0, a115 = 0, a40 = a40, a68 = 0, a92 = -\frac{884}{45387} a40^2 \right\} \quad (71)$$

**G > Branch[3]:=subs(RootOf(218489\*\_Z^2-515, label = \_L114)=b,branch[3]);**

$$\text{Branch}_3 := \left\{ a10 = \frac{294}{5329} a68^2, a105 = \frac{221}{3} b a68, a110 = -\frac{367}{73} b a68^2, a115 = -\frac{294}{73} a68, a40 = 0, a68 = a68, a92 = -\frac{59941}{655467} a68^2 \right\} \quad (72)$$

**G > Branch[4]:=subs(RootOf(218489\*\_Z^2-515, label = \_L116)=b,branch[4]);**

$$\text{Branch}_4 := \left\{ a10 = \frac{50470}{655467} a40^2, a105 = -\frac{294}{73} a40, a110 = -\frac{367}{73} b a40^2, a115 = \frac{221}{3} b a40, a40 = a40, a68 = 0, a92 = -\frac{6359}{655467} a40^2 \right\} \quad (73)$$

**G > Branch[5]:=subs(RootOf(1966401\*\_Z^3+15449939\*\_Z^2\*a68+(-25153115\*a40^2+28761432\*a68^2)\*\_Z-46740837\*a40^2\*a68-6309828\*a68^3)=b,branch[5]);**

$$\begin{aligned}
\text{Branch}_5 := & \left\{ a10 = \frac{294}{48841} b^2 + \frac{588}{48841} b a68 + \frac{294}{48841} a68^2, a105 = -\frac{1}{81549} \frac{-16133 a40^2 - 21462 a68^2 + 103157 a68 b + 26937 b^2}{a40}, \right. \\
& a110 = \frac{367}{438543339} \frac{-179231 a40^2 a68 - 81549 a40^2 b - 21462 a68^3 + 103157 a68^2 b + 26937 a68 b^2}{a40}, a115 = b, a40 = a40, a68 = a68, \\
& \left. a92 = \frac{4591}{6007443} b^2 + \frac{61215902}{2216746467} b a68 - \frac{884}{45387} a40^2 + \frac{5448793}{738915489} a68^2 \right\}
\end{aligned} \quad (74)$$

Now we initialize the solutions to inspect them. Case 1:

```

G > nbrak2:=DGsimplify(subs(branch[1],subs(jacgroblinsol,genbrak2))):
g > ngiso2:=DGsimplify(subs(branch[1],subs(jacgroblinsol,gisoten2))):
ngiso2 :=  $\left[ -(D_{w2} dw2) - ((2 D_{w3}) dw3) + D_{w4} dw4 + D_{w5} dw5 - (D_{w6} dw6) - (D_{w7} dw7), \left( \frac{98 a68}{123} D_{w1} \right) dw4 + D_{w2} dw1 \right.$  (75)
 $\left. - \left( \left( \frac{16 a68}{41} D_{w2} \right) dw8 \right) + \left( \frac{221 a68}{738} D_{w3} \right) dw7 + D_{w6} dw8 + D_{w7} dw9 - (D_{w8} dw4) - (D_{w9} dw5), \right.$ 
 $\left. - \left( \left( \frac{8 a68}{123} D_{w2} \right) dw5 \right) + (2 D_{w3}) dw1 - \left( \left( \frac{25 a68}{123} D_{w3} \right) dw8 \right) - ((6 D_{w6}) dw5) + (6 D_{w7}) dw4 \right]$ 

G > DGsetup(LieAlgebraData(cohom_algfromten(nbrak2,ngiso2),G));
Lie algebra: G (76)

G > LD:=LeviDecomposition();
LD :=  $\left[ \left[ e1 + \frac{369}{148 a68} e8, e2 + \frac{369}{4 a68} e6, e3, e5, e7, e9 \right], \left[ e1 - \left( \frac{123}{98 a68} e8 \right), e2 - \left( \frac{123}{146 a68} e6 \right), e4 \right] \right]$  (77)

G > LieBracket(LD[2][1],LD[1][6]);
 $\frac{221}{294} e9$  (78)

G > DGsetup(LieAlgebraData(LD[1],A));
Lie algebra: A (79)

A > MultiplicationTable();
 $\left[ [e1, e2] = -\frac{221}{74} e2, [e1, e3] = -\frac{221}{148} e3, [e1, e4] = -\frac{221}{148} e4, [e1, e5] = -\frac{221}{148} e5, [e1, e6] = -\frac{221}{148} e6, [e3, e4] = -\frac{8}{123} a68 e2, [e5, \right.$  (80)
 $\left. e6] = -\frac{884}{45387} a68^2 e2 \right]$ 

G > Query("Jacobi");
true (81)

G > ChangeFrame(G);
A (82)

G > Jten:=evalDG(add(e||(2*i) &t theta||(2*i+1) - e||(2*i+1) &t theta||(2*i),i=2..4)):Pf:=(x,i)
->ContractIndices(mproj_ten,convert(x,DGtensor),[[2,i]]):NJ:=Pf(Pf(Pm(TensorBrackets(Jten,
Jten,"Frolicher-Nijenhuis"),1),2),3):
G > DGImageSpace(x->ContractIndices(x,NJ,[[1,1],[2,2]]),GenerateTensors([DGinfo(G,
"FrameBaseVectors"),DGinfo(G,"FrameBaseVectors")])):nops(%);

```

$$\left[ \frac{1768 a68}{369} e8, -\left( \frac{1768 a68}{369} e9 \right), -\left( \frac{1768 a68}{369} e4 \right), \frac{1768 a68}{369} e5, \frac{1768 a68}{369} e6, -\left( \frac{1768 a68}{369} e7 \right) \right]$$

6

(83)

Case 2:

```
G > nbrak2:=DGsimplify(subs(branch[2],subs(jacgroblinsol,genbrak2))):
g > ngiso2:=DGsimplify(subs(branch[2],subs(jacgroblinsol,gisoten2))):
```

$$\begin{aligned} \text{ngiso2} := & \left[ -(D_{w2} dw2) - ((2 D_{w3}) dw3) + D_{w4} dw4 + D_{w5} dw5 - (D_{w6} dw6) - (D_{w7} dw7), \left( \frac{98 a40}{123} D_{w1} \right) dw5 + D_{w2} dw1 \right. \\ & - \left( \left( \frac{16 a40}{41} D_{w2} \right) dw9 \right) - \left( \left( \frac{221 a40}{738} D_{w3} \right) dw6 \right) + D_{w6} dw8 + D_{w7} dw9 - (D_{w8} dw4) - (D_{w9} dw5), \\ & \left. \left( \frac{8 a40}{123} D_{w2} \right) dw4 + (2 D_{w3}) dw1 - \left( \left( \frac{25 a40}{123} D_{w3} \right) dw9 \right) - ((6 D_{w6}) dw5) + (6 D_{w7}) dw4 \right] \end{aligned}$$
(84)

```
G > DGsetup(LieAlgebraData(cohom_algfromten(nbrak2,ngiso2),G));
Lie algebra: G
```

(85)

```
G > LD:=LeviDecomposition();
```

$$LD := \left[ \left[ e1 + \frac{369}{148 a40} e9, e2 + \frac{369}{4 a40} e7, e3, e4, e6, e8 \right], \left[ e1 - \left( \frac{123}{98 a40} e9 \right), e2 - \left( \frac{123}{146 a40} e7 \right), e5 \right] \right]$$
(86)

```
G > LieBracket(LD[2][1],LD[1][5]);
```

$$-\left( \frac{221}{294} e6 \right)$$
(87)

```
G > DGsetup(LieAlgebraData(LD[1],A));
Lie algebra: A
```

(88)

```
A > MultiplicationTable();
```

$$\begin{aligned} [e1, e2] = & -\frac{221}{74} e2, [e1, e3] = -\frac{221}{148} e3, [e1, e4] = -\frac{221}{148} e4, [e1, e5] = -\frac{221}{148} e5, [e1, e6] = -\frac{221}{148} e6, [e3, e4] = \frac{8}{123} a40 e2, [e5, e6] \\ = & -\frac{884}{45387} a40^2 e2 \end{aligned}$$
(89)

```
G > Query("Jacobi");
true
```

(90)

```
G > ChangeFrame(G);
A
```

(91)

```
G > Jten:=evalDG(add(e||(2*i) &t theta||(2*i+1) - e||(2*i+1) &t theta||(2*i),i=2..4)):Pf:=(x,i)
```

```
->ContractIndices(mproj_ten,convert(x,DGtensor),[[2,i]]):NJ:=Pf(Pf(Pm(TensorBrackets(Jten,
Jten,"Frolicher-Nijenhuis"),1),2),3):
```

```
G > DGImageSpace(x->ContractIndices(x,NJ,[[1,1],[2,2]]),GenerateTensors([DGinfo(G,
"FrameBaseVectors"),DGinfo(G,"FrameBaseVectors")]);nops(%);
```

$$\left[ -\left( \frac{1768 a40}{369} e9 \right), -\left( \frac{1768 a40}{369} e8 \right), \frac{1768 a40}{369} e5, \frac{1768 a40}{369} e4, -\left( \frac{1768 a40}{369} e7 \right), -\left( \frac{1768 a40}{369} e6 \right) \right]$$

6

(92)

Case 3:

```
G > unassign('b');
```

```
G > nbrak2:=DGsimplify(subs(Branch[3],subs(jacgroblinsol,genbrak2))):
```

```
G > ngiso2:=DGsimplify(subs(Branch[3],subs(jacgroblinsol,gisoten2))):
```

```
ngiso2 := [ -(D_w2 dw2) - ((2 D_w3) dw3) + D_w4 dw4 + D_w5 dw5 - (D_w6 dw6) - (D_w7 dw7), -\left( \left( \frac{147 a68}{73} D_w1 \right) dw4 \right) \quad (93)
```

$$+ (49 b a68 D_w1) dw5 + D_w2 dw1 + \left( \frac{72 a68}{73} D_w2 \right) dw8 - ((24 b a68 D_w2) dw9) - \left( \left( \frac{221 b a68}{12} D_w3 \right) dw6 \right)$$

$$- \left( \left( \frac{221 a68}{292} D_w3 \right) dw7 \right) + D_w6 dw8 + D_w7 dw9 - (D_w8 dw4) - (D_w9 dw5), (4 b a68 D_w2) dw4 + \left( \frac{12 a68}{73} D_w2 \right) dw5$$

$$+ (2 D_w3) dw1 + \left( \frac{75 a68}{146} D_w3 \right) dw8 - \left( \left( \frac{25 b a68}{2} D_w3 \right) dw9 \right) - ((6 D_w6) dw5) + (6 D_w7) dw4 ]$$

```
G > DGsetup(LieAlgebraData(cohom_algfromten(nbrak2,ngiso2),G));
```

*Lie algebra: G*

(94)

```
G > Query({b},"Jacobi")[2]:Groebner[Basis](%,'asrtgaa');solve(%);
```

$[218489 a68^2 b^2 - 515 a68^2]$

$\{a68=0, b=b\}, \left\{ a68=a68, b=\frac{1}{2993} \sqrt{21115} \right\}, \left\{ a68=a68, b=-\frac{1}{2993} \sqrt{21115} \right\}$  (95)

```
G > b:=(1/2993)*sqrt(21115);
```

$b := \frac{1}{2993} \sqrt{21115}$  (96)

```
G > LD:=LeviDecomposition();
```

$LD := \left[ \left[ e1 + \frac{219 \sqrt{21115}}{38110 a68} e9, e2 + \frac{219 \sqrt{21115}}{1030 a68} e7, e3, e4 + \frac{3 \sqrt{21115}}{515} e5, e6 + \frac{3 \sqrt{21115}}{515} e7, e8 + \frac{3 \sqrt{21115}}{515} e9 \right], \left[ e1 \right. \right. \quad (97)$

$$+ \frac{8979}{43316 a68} e8 - \left( \frac{73 \sqrt{21115}}{43316 a68} e9 \right), e2 + \frac{123}{884 a68} e6 - \left( \frac{\sqrt{21115}}{884 a68} e7 \right), e4 - \left( \frac{\sqrt{21115}}{123} e5 \right) \Big] \Big]$$

**G > LieBracket(LD[2][1],LD[1][5]);**

$$- \left( \frac{221}{294} e6 \right) - \left( \frac{221 \sqrt{21115}}{50470} e7 \right) \quad (98)$$

**G > DGsetup(LieAlgebraData(LD[1],A));**

*Lie algebra: A*

**A > MultiplicationTable();**

$$\begin{aligned} [e1, e2] &= -\frac{26937}{1030} \frac{e5}{a68} + \frac{17017}{76220} e2, [e1, e3] = -\frac{221}{148} e3, [e1, e4] = -\frac{221}{148} e4, [e1, e5] = -\frac{179231}{38110} e5 + \frac{293046}{1391015} a68 e2, [e1, e6] = \\ &= -\frac{221}{148} e6, [e2, e6] = \frac{244647}{2060} e5 - \frac{293046}{37595} a68 e2, [e3, e4] = -\frac{18}{515} \sqrt{21115} e5 + \frac{3536}{1541395} \sqrt{21115} a68 e2, [e5, e6] \\ &= \frac{293046}{37595} a68 e5 - \frac{172701776}{337565505} a68^2 e2 \end{aligned} \quad (100)$$

**G > DGsetup(LieAlgebraData([e1,evalDG((3536\*sqrt(21115)\*a68\*(1/1541395))\*e2-(18\*sqrt(21115)\*(1/515))\*e5),e3,e4,e5,e6],A));**

*Lie algebra: A*

(101)

**A > MultiplicationTable();**

$$\begin{aligned} [e1, e2] &= -\frac{221}{74} e2, [e1, e3] = -\frac{221}{148} e3, [e1, e4] = -\frac{221}{148} e4, [e1, e5] = -\frac{221}{148} e5 + \frac{663}{152440} \sqrt{21115} e2, [e1, e6] = -\frac{221}{148} e6, [e3, e4] \\ &= e2, [e5, e6] = -\frac{48841}{4624185} \sqrt{21115} a68 e2 \end{aligned} \quad (102)$$

**A > LieBracket(e1,evalDG(e5+k\*e2));**

$$- \left( \left( -\frac{663 \sqrt{21115}}{152440} + \frac{221 k}{74} \right) e2 \right) - \left( \frac{221}{148} e5 \right) \quad (103)$$

**A > solve(221\*k\*(1/74)-663\*sqrt(21115)\*(1/152440),k);**

$$\frac{3}{2060} \sqrt{21115} \quad (104)$$

**G > ChangeFrame(G);**

*G*

(105)

**G > Jten:=evalDG(add(e|| (2\*i) &t theta|| (2\*i+1) - e|| (2\*i+1) &t theta|| (2\*i),i=2..4)):Pf:=(x,i)**



```
->ContractIndices(mproj_ten,convert(x,DGtensor),[[2,i]]):NJ:=Pf(Pf(Pm(TensorBrackets(Jten,
Jten,"Frolicher-Nijenhuis"),1),2),3):
```

```
G > DGImageSpace(x->ContractIndices(x,NJ,[[1,1],[2,2]]),GenerateTensors([DGinfo(G,
"FrameBaseVectors"),DGinfo(G,"FrameBaseVectors")]);nops(%);
```

$$\left[ \frac{1176 a68}{73} e8 + \frac{592 \sqrt{21115} a68}{8979} e9, \frac{592 \sqrt{21115} a68}{8979} e8 - \left( \frac{1176 a68}{73} e9 \right), - \left( \frac{1176 a68}{73} e4 \right) - \left( \frac{592 \sqrt{21115} a68}{8979} e5 \right), \right. \\ \left. - \left( \frac{592 \sqrt{21115} a68}{8979} e4 \right) + \frac{1176 a68}{73} e5, \frac{1176 a68}{73} e6 + \frac{592 \sqrt{21115} a68}{8979} e7, \frac{592 \sqrt{21115} a68}{8979} e6 - \left( \frac{1176 a68}{73} e7 \right) \right]$$

6

(106)

Case 4:

```
G > unassign('b');
```

```
G > nbrak2:=DGsimplify(subs(Branch[4],subs(jacgroblinsol,genbrak2))):
```

```
g > ngiso2:=DGsimplify(subs(Branch[4],subs(jacgroblinsol,gisoten2))):
```

$$\text{ngiso2} := \left[ - (D_{w2} dw2) - ((2 D_{w3}) dw3) + D_{w4} dw4 + D_{w5} dw5 - (D_{w6} dw6) - (D_{w7} dw7), (49 b a40 D_{w1}) dw4 \right. \\ \left. - \left( \left( \frac{147 a40}{73} D_{w1} \right) dw5 \right) + D_{w2} dw1 - ((24 b a40 D_{w2}) dw8) + \left( \frac{72 a40}{73} D_{w2} \right) dw9 + \left( \frac{221 a40}{292} D_{w3} \right) dw6 \right. \\ \left. + \left( \frac{221 b a40}{12} D_{w3} \right) dw7 + D_{w6} dw8 + D_{w7} dw9 - (D_{w8} dw4) - (D_{w9} dw5), - \left( \left( \frac{12 a40}{73} D_{w2} \right) dw4 \right) \right. \\ \left. - ((4 b a40 D_{w2}) dw5) + (2 D_{w3}) dw1 - \left( \left( \frac{25 b a40}{2} D_{w3} \right) dw8 \right) + \left( \frac{75 a40}{146} D_{w3} \right) dw9 - ((6 D_{w6}) dw5) \right. \\ \left. + (6 D_{w7}) dw4 \right]$$

(107)

```
G > DGsetup(LieAlgebraData(cohom_algfromten(nbrak2,ngiso2),G));
```

Lie algebra: G

(108)

```
G > Query({b},"Jacobi")[2]:Groebner[Basis](%,'asrtgaa');solve(%);
```

$$\begin{aligned} & [218489 a40^2 b^2 - 515 a40^2] \\ & \{a40=0, b=b\}, \left\{ a40=a40, b=\frac{1}{2993} \sqrt{21115} \right\}, \left\{ a40=a40, b=-\frac{1}{2993} \sqrt{21115} \right\} \end{aligned}$$

(109)

```
G > b:=(1/2993)*sqrt(21115);
```

$$b := \frac{1}{2993} \sqrt{21115}$$

(110)

G > ChangeFrame(G);

G

(111)

G > LD:=LeviDecomposition();

$$LD := \left[ \left[ e1 - \left( \frac{73}{74 a40} e9 \right), e2 - \left( \frac{73}{2 a40} e7 \right), e3, e4 + \frac{\sqrt{21115}}{123} e5, e6 + \frac{\sqrt{21115}}{123} e7, e8 + \frac{\sqrt{21115}}{123} e9 \right], \left[ e1 + \frac{73}{147 a40} e9, e2 - \left( \frac{3066 \sqrt{21115}}{817921 a40} e6 \right) + \frac{6608544}{5725447 a40} e7, e4 + \frac{98 \sqrt{21115}}{21115} e5 \right] \right] \quad (112)$$

G > LieBracket(LD[2][1],LD[1][5]);

$$\frac{195364 \sqrt{21115} a40}{162349299} e2 + \frac{884}{369} e6 - \left( \frac{442 \sqrt{21115}}{18081} e7 \right) \quad (113)$$

G > DGsetup(LieAlgebraData(LD[1],A));

Lie algebra: A

(114)

A > MultiplicationTable();

$$\begin{aligned} [e1, e2] &= \frac{3577}{6068} \frac{\sqrt{21115} e5}{a40} + \frac{59449}{18204} e2, [e1, e3] = -\frac{221}{148} e3, [e1, e4] = -\frac{221}{148} e4, [e1, e5] = -\frac{70499}{9102} e5 \\ &- \frac{97682}{40863429} \sqrt{21115} a40 e2, [e1, e6] = -\frac{221}{148} e6, [e2, e6] = \frac{113815}{492} e5 + \frac{97682}{1104417} \sqrt{21115} a40 e2, [e3, e4] = -\frac{2}{41} \sqrt{21115} e5 \\ &- \frac{3536}{8979} a40 e2, [e5, e6] = -\frac{97682}{1104417} \sqrt{21115} a40 e5 - \frac{172701776}{241867323} a40^2 e2 \end{aligned} \quad (115)$$

G > ChangeFrame(G);

G

(116)

G > Jten:=evalDG(add(e||(2\*i) &t theta||(2\*i+1) - e||(2\*i+1) &t theta||(2\*i),i=2..4)):Pf:=(x,i) ->ContractIndices(mproj\_ten,convert(x,DGtensor),[[2,i]]):NJ:=Pf(Pf(Pm(TensorBrackets(Jten, Jten,"Frolicher-Nijenhuis"),1),2),3):

G > DGImageSpace(x->ContractIndices(x,NJ,[[1,1],[2,2]]),GenerateTensors([DGinfo(G, "FrameBaseVectors"),DGinfo(G,"FrameBaseVectors")])):nops(%);

$$\begin{aligned} &\left[ -\left( \frac{592 \sqrt{21115} a40}{8979} e8 \right) - \left( \frac{1176 a40}{73} e9 \right), -\left( \frac{1176 a40}{73} e8 \right) + \frac{592 \sqrt{21115} a40}{8979} e9, \frac{592 \sqrt{21115} a40}{8979} e4 + \frac{1176 a40}{73} e5, \right. \\ &\left. \frac{1176 a40}{73} e4 - \left( \frac{592 \sqrt{21115} a40}{8979} e5 \right), -\left( \frac{592 \sqrt{21115} a40}{8979} e6 \right) - \left( \frac{1176 a40}{73} e7 \right), -\left( \frac{1176 a40}{73} e6 \right) + \frac{592 \sqrt{21115} a40}{8979} e7 \right] \end{aligned}$$

(117)

It is easy to see that the first four families are isomorphic, and they admit almost complex structures with non-degenerate Nijenhuis tensors. Their visible differences come from the embedding of the isotropy algebra. Case 5:

```
> unassign('b');
G > nbrak2:=DGsimplify(subs(Branch[5],subs(jacgroblinsol,genbrak2))):
g > ngiso2:=DGsimplify(subs(Branch[5],subs(jacgroblinsol,gisoten2))):
G > DGsetup(LieAlgebraData(cohom_algfromten(nbrak2,ngiso2),G));
```

*Lie algebra: G* (118)

```
G > Query({b}, "Jacobi")[2]:solve(%,b);
{b:=RootOf(1966401 _Z^3 + 15449939 _Z^2 a68 + (-25153115 a40^2 + 28761432 a68^2) _Z - 46740837 a40^2 a68 - 6309828 a68^3)}
```

(119)

```
G > b:=RootOf(1966401*_Z^3+15449939*_Z^2*a68+(-25153115*a40^2+28761432*a68^2)*_Z-46740837*a40^2*
a68-6309828*a68^3);
b:=RootOf(1966401 _Z^3 + 15449939 _Z^2 a68 + (-25153115 a40^2 + 28761432 a68^2) _Z - 46740837 a40^2 a68 - 6309828 a68^3)
```

(120)

```
G > DS:=Series("Derived"):map(x->nops(x),%);
```

[9, 8, 8] (121)

```
G > rad:=Radical():nops(%)
```

6 (122)

We omit the full computation of branch 5 for now.

Section 4: all solutions are equivalent.

```
> data:=[[q1,q2]=2*q2,seq([q1,q|i]=q|i,i=3..6),[q3,q4]=q2,[q5,q6]=q2],[seq(q|i,i=1..6)];
data:=[[q1,q2]=2 q2,[q1,q3]=q3,[q1,q4]=q4,[q1,q5]=q5,[q1,q6]=q6,[q3,q4]=q2,[q5,q6]=q2],[q1,q2,q3,q4,q5,q6]
```

(123)

We start with the normal form of the radical from our solutions.

```
> SData:=LieAlgebraData(data,S);
SData:=[[e1,e2]=2 e2,[e1,e3]=e3,[e1,e4]=e4,[e1,e5]=e5,[e1,e6]=e6,[e3,e4]=e2,[e5,e6]=e2]
```

(124)

```
> DGsetup(SData);
```

*Lie algebra: S* (125)

```
S > Query("Jacobi");
```

*true* (126)

```
S > outder:=Derivations("Outer");nops(%)
```



$$\begin{bmatrix} 0 & 0 & 0 & 0 & 0 & 0 \\ 0 & 0 & 0 & 0 & 0 & 0 \\ 0 & 0 & 0 & 0 & 0 & 0 \\ 0 & 0 & 0 & 0 & 1 & 0 \\ 0 & 0 & 0 & 0 & 0 & 0 \\ 0 & 0 & 1 & 0 & 0 & 0 \end{bmatrix}
 \begin{bmatrix} 0 & 0 & 0 & 0 & 0 & 0 \\ 0 & 0 & 0 & 0 & 0 & 0 \\ 0 & 0 & 0 & 0 & 0 & 0 \\ 0 & 0 & 0 & 0 & 0 & 1 \\ 0 & 0 & -1 & 0 & 0 & 0 \\ 0 & 0 & 0 & 0 & 0 & 0 \end{bmatrix}
 \begin{bmatrix} 0 & 0 & 0 & 0 & 0 & 0 \\ 0 & 0 & 0 & 0 & 0 & 0 \\ 0 & 0 & 0 & 0 & 0 & 0 \\ 0 & 0 & 0 & 0 & 0 & 0 \\ 0 & 0 & 0 & 0 & 0 & 1 \\ 0 & 0 & 0 & 0 & 0 & 0 \end{bmatrix}
 \begin{bmatrix} 0 & 0 & 0 & 0 & 0 & 0 \\ 0 & 0 & 0 & 0 & 0 & 0 \\ 0 & 0 & 0 & 0 & 0 & 0 \\ 0 & 0 & 0 & 0 & 0 & 0 \\ 0 & 0 & 0 & 0 & 0 & 0 \\ 0 & 0 & 0 & 0 & 1 & 0 \end{bmatrix}
 \begin{bmatrix} 0 & 0 & 0 & 0 & 0 & 0 \\ 0 & 0 & 0 & 0 & 0 & 0 \\ 0 & 0 & -1 & 0 & 0 & 0 \\ 0 & 0 & 0 & 1 & 0 & 0 \\ 0 & 0 & 0 & 0 & 1 & 0 \\ 0 & 0 & 0 & 0 & 0 & -1 \end{bmatrix}$$

11

(128

`S > 2*outder[1]+2*outder[2]+1*outder[11];`

$$\begin{bmatrix} 0 & 0 & 0 & 0 & 0 & 0 \\ 0 & 2 & 0 & 0 & 0 & 0 \\ 0 & 0 & 1 & 0 & 0 & 0 \\ 0 & 0 & 0 & 1 & 0 & 0 \\ 0 & 0 & 0 & 0 & 1 & 0 \\ 0 & 0 & 0 & 0 & 0 & 1 \end{bmatrix}$$

(129

This linear combination of outer derivations is actually inner.

`S > innder:=Derivations("Inner");`

(130

$$innder := \left[ \begin{bmatrix} 0 & 0 & 0 & 0 & 0 & 0 \\ 1 & 0 & 0 & 0 & 0 & 0 \\ 0 & 0 & 0 & 0 & 0 & 0 \\ 0 & 0 & 0 & 0 & 0 & 0 \\ 0 & 0 & 0 & 0 & 0 & 0 \\ 0 & 0 & 0 & 0 & 0 & 0 \end{bmatrix}, \begin{bmatrix} 0 & 0 & 0 & 0 & 0 & 0 \\ 0 & 1 & 0 & 0 & 0 & 0 \\ 0 & 0 & \frac{1}{2} & 0 & 0 & 0 \\ 0 & 0 & 0 & \frac{1}{2} & 0 & 0 \\ 0 & 0 & 0 & 0 & \frac{1}{2} & 0 \\ 0 & 0 & 0 & 0 & 0 & \frac{1}{2} \end{bmatrix}, \begin{bmatrix} 0 & 0 & 0 & 0 & 0 & 0 \\ 0 & 0 & 1 & 0 & 0 & 0 \\ 0 & 0 & 0 & 0 & 0 & 0 \\ 1 & 0 & 0 & 0 & 0 & 0 \\ 0 & 0 & 0 & 0 & 0 & 0 \\ 0 & 0 & 0 & 0 & 0 & 0 \end{bmatrix}, \begin{bmatrix} 0 & 0 & 0 & 0 & 0 & 0 \\ 0 & 0 & 0 & 1 & 0 & 0 \\ -1 & 0 & 0 & 0 & 0 & 0 \\ 0 & 0 & 0 & 0 & 0 & 0 \\ 0 & 0 & 0 & 0 & 0 & 0 \\ 0 & 0 & 0 & 0 & 0 & 0 \end{bmatrix}, \begin{bmatrix} 0 & 0 & 0 & 0 & 0 & 0 \\ 0 & 0 & 0 & 0 & 1 & 0 \\ 0 & 0 & 0 & 0 & 0 & 0 \\ 0 & 0 & 0 & 0 & 0 & 0 \\ 0 & 0 & 0 & 0 & 0 & 0 \\ 1 & 0 & 0 & 0 & 0 & 0 \end{bmatrix} \right], \quad (130)$$

$$\begin{bmatrix} 0 & 0 & 0 & 0 & 0 & 0 \\ 0 & 0 & 0 & 0 & 0 & 1 \\ 0 & 0 & 0 & 0 & 0 & 0 \\ 0 & 0 & 0 & 0 & 0 & 0 \\ -1 & 0 & 0 & 0 & 0 & 0 \\ 0 & 0 & 0 & 0 & 0 & 0 \end{bmatrix}$$

---

**S > GData:=simplify(LieAlgebraData(outder,G));**

**GData :=** [[e1, e3] = -e3, [e1, e5] = -e5, [e1, e6] = e6, [e1, e7] = e7, [e1, e9] = -e9, [e1, e10] = e10, [e2, e3] = 2 e3, [e2, e4] = e4, [e2, e5] = e5, [e2, e6] = -2 e6, [e2, e7] = -e7, [e2, e8] = -e8, [e3, e6] = e2, [e3, e7] = e4, [e3, e8] = e5, [e3, e11] = 2 e3, [e4, e5] = 2 e3, [e4, e6] = -e7, [e4, e7] = -2 e10, [e4, e8] = e11, [e4, e9] = e5, [e4, e11] = 2 e4, [e5, e6] = -e8, [e5, e7] = e11 + 2 e2, [e5, e8] = 2 e9, [e5, e10] = e4, [e6, e11] = -2 e6, [e7, e8] = -2 e6, [e7, e9] = e8, [e8, e10] = e7, [e8, e11] = -2 e8, [e9, e10] = e11 + e2, [e9, e11] = -2 e9, [e10, e11] = 2 e10] (131)

---

**S > DGsetup(GData);**

(132)

*Lie algebra: G*

(132)

```
S > LeviDecomposition();
```

$$\left[ \left[ e1 + e2 + \frac{1}{2} e11 \right], [e2, e3, e4, e5, e6, e7, e8, e9, e10, e11] \right]$$

(133)

```
S > sl2:=[4*outder[2]+outder[11]];
```

$$sl2 := \begin{bmatrix} 0 & 0 & 0 & 0 & 0 & 0 \\ 0 & 0 & 0 & 0 & 0 & 0 \\ 0 & 0 & 3 & 0 & 0 & 0 \\ 0 & 0 & 0 & -3 & 0 & 0 \\ 0 & 0 & 0 & 0 & 1 & 0 \\ 0 & 0 & 0 & 0 & 0 & -1 \end{bmatrix}$$

(134)

We need to find the correct conjugacy class of sl2 to act on our radical. This should be irreducible.

```
R6 > DGsetup(LieAlgebraData(outder,O));
```

*Lie algebra: O*

(135)

```
O > interface(rtablesize=11);
```

10

(136)

```
O > h:=evalDG(4*e2+e11);
```

$$h := 4 e2 + e11$$

(137)

```
R6 > E:=evalDG(a1*e4+a2*e9);
```

$$E := a1 e4 + a2 e9$$

(138)

```
R6 > F:=evalDG(b1*e8+b2*e10);
```

$$F := b1 e8 + b2 e10$$

(139)

```
R6 > compbas:=ComplementaryBasis([h,E,F],DGinfo(O,"FrameBaseVectors"));
```

$$compbas := [e1, e2, e3, e4, e5, e6, e7, e8]$$

(140)

```
O > GetComponents(LieBracket(E,F),[op([h,E,F]),op(compbas)])[4..11];
```

$$[0, -4 a1 b1 - 3 a2 b2, 0, 0, 0, 0, 0, 0]$$

(141)

```
O > GetComponents(LieBracket(E,F),[op([h,E,F]),op(compbas)])[1..3];
```

$$[a1 b1 + a2 b2, 0, 0]$$

(142)

```
O > ssol:=solve({-4*a1*b1-3*a2*b2,a1*b1+a2*b2-1});
```

(143)

$$ssol := \left\{ a1 = -\frac{3}{b1}, a2 = \frac{4}{b2}, b1 = b1, b2 = b2 \right\} \quad (143)$$

```
O > E:=DGsimplify(subs({b1=3,b2=4},subs(ssol,E)));F:=DGsimplify(subs({b1=3,b2=4},subs(ssol,F)));
      E := -e4 + e9
      F := 3 e8 + 4 e10
```

(144)

```
O > HH:=add(GetComponents(h,DGinfo(O,"FrameBaseVectors"))[i]*outder[i],i=1..11):EE:=add
      (GetComponents(E,DGinfo(O,"FrameBaseVectors"))[i]*outder[i],i=1..11):FF:=add(GetComponents(F,
      DGinfo(O,"FrameBaseVectors"))[i]*outder[i],i=1..11):
```

```
O > sl2:=[HH,
      EE,FF];
```

$$sl2 := \left[ \begin{bmatrix} 0 & 0 & 0 & 0 & 0 & 0 \\ 0 & 0 & 0 & 0 & 0 & 0 \\ 0 & 0 & 3 & 0 & 0 & 0 \\ 0 & 0 & 0 & -3 & 0 & 0 \\ 0 & 0 & 0 & 0 & 1 & 0 \\ 0 & 0 & 0 & 0 & 0 & -1 \end{bmatrix}, \begin{bmatrix} 0 & 0 & 0 & 0 & 0 & 0 \\ 0 & 0 & 0 & 0 & 0 & 0 \\ 0 & 0 & 0 & 0 & -1 & 0 \\ 0 & 0 & 0 & 0 & 0 & 0 \\ 0 & 0 & 0 & 0 & 0 & 1 \\ 0 & 0 & 0 & 1 & 0 & 0 \end{bmatrix}, \begin{bmatrix} 0 & 0 & 0 & 0 & 0 & 0 \\ 0 & 0 & 0 & 0 & 0 & 0 \\ 0 & 0 & 0 & 0 & 0 & 0 \\ 0 & 0 & 0 & 0 & 0 & 3 \\ 0 & 0 & -3 & 0 & 0 & 0 \\ 0 & 0 & 0 & 0 & 4 & 0 \end{bmatrix} \right] \quad (145)$$

We can see that this is an irreducible action on  $V^4$ .

```
S > LieAlgebraData(sl2);
```

$$[[e1, e2] = 2 e2, [e1, e3] = -2 e3, [e2, e3] = e1] \quad (146)$$

```
S > Sym:=[op(innder),op(sl2)];
```

(147)



$$Sym := \left[ \begin{bmatrix} 0 & 0 & 0 & 0 & 0 & 0 \\ 1 & 0 & 0 & 0 & 0 & 0 \\ 0 & 0 & 0 & 0 & 0 & 0 \\ 0 & 0 & 0 & 0 & 0 & 0 \\ 0 & 0 & 0 & 0 & 0 & 0 \\ 0 & 0 & 0 & 0 & 0 & 0 \end{bmatrix}, \begin{bmatrix} 0 & 0 & 0 & 0 & 0 & 0 \\ 0 & 1 & 0 & 0 & 0 & 0 \\ 0 & 0 & \frac{1}{2} & 0 & 0 & 0 \\ 0 & 0 & 0 & \frac{1}{2} & 0 & 0 \\ 0 & 0 & 0 & 0 & \frac{1}{2} & 0 \\ 0 & 0 & 0 & 0 & 0 & \frac{1}{2} \end{bmatrix}, \begin{bmatrix} 0 & 0 & 0 & 0 & 0 & 0 \\ 0 & 0 & 1 & 0 & 0 & 0 \\ 0 & 0 & 0 & 0 & 0 & 0 \\ 1 & 0 & 0 & 0 & 0 & 0 \\ 0 & 0 & 0 & 0 & 0 & 0 \\ 0 & 0 & 0 & 0 & 0 & 0 \end{bmatrix}, \begin{bmatrix} 0 & 0 & 0 & 0 & 0 & 0 \\ 0 & 0 & 0 & 1 & 0 & 0 \\ -1 & 0 & 0 & 0 & 0 & 0 \\ 0 & 0 & 0 & 0 & 0 & 0 \\ 0 & 0 & 0 & 0 & 0 & 0 \\ 0 & 0 & 0 & 0 & 0 & 0 \end{bmatrix}, \begin{bmatrix} 0 & 0 & 0 & 0 & 0 & 0 \\ 0 & 0 & 0 & 0 & 1 & 0 \\ 0 & 0 & 0 & 0 & 0 & 0 \\ 0 & 0 & 0 & 0 & 0 & 0 \\ 0 & 0 & 0 & 0 & 0 & 0 \\ 1 & 0 & 0 & 0 & 0 & 0 \end{bmatrix} \right], \quad (147)$$

$$\left[ \begin{bmatrix} 0 & 0 & 0 & 0 & 0 & 0 \\ 0 & 0 & 0 & 0 & 0 & 1 \\ 0 & 0 & 0 & 0 & 0 & 0 \\ 0 & 0 & 0 & 0 & 0 & 0 \\ -1 & 0 & 0 & 0 & 0 & 0 \\ 0 & 0 & 0 & 0 & 0 & 0 \end{bmatrix}, \begin{bmatrix} 0 & 0 & 0 & 0 & 0 & 0 \\ 0 & 0 & 0 & 0 & 0 & 0 \\ 0 & 0 & 3 & 0 & 0 & 0 \\ 0 & 0 & 0 & -3 & 0 & 0 \\ 0 & 0 & 0 & 0 & 1 & 0 \\ 0 & 0 & 0 & 0 & 0 & -1 \end{bmatrix}, \begin{bmatrix} 0 & 0 & 0 & 0 & 0 & 0 \\ 0 & 0 & 0 & 0 & 0 & 0 \\ 0 & 0 & 0 & 0 & -1 & 0 \\ 0 & 0 & 0 & 0 & 0 & 0 \\ 0 & 0 & 0 & 0 & 0 & 1 \\ 0 & 0 & 0 & 1 & 0 & 0 \end{bmatrix}, \begin{bmatrix} 0 & 0 & 0 & 0 & 0 & 0 \\ 0 & 0 & 0 & 0 & 0 & 0 \\ 0 & 0 & 0 & 0 & 0 & 0 \\ 0 & 0 & 0 & 0 & 0 & 3 \\ 0 & 0 & -3 & 0 & 0 & 0 \\ 0 & 0 & 0 & 0 & 4 & 0 \end{bmatrix} \right]$$

Now take the semi-direct product of our  $sl_2$  and the radical to get the symmetry algebra  $g$ .

**S > DGsetup(LieAlgebraData(Sym,sym));**

*Lie algebra: sym*

**sym > LieAlgebraData([e1,evalDG(2\*e2),e3,e4,e5,e6,e7,e8,e9],sym);**

$[[e1, e2] = -2 e1, [e2, e3] = e3, [e2, e4] = e4, [e2, e5] = e5, [e2, e6] = e6, [e3, e4] = -2 e1, [e3, e7] = 3 e3, [e3, e8] = -e5, [e4, e7] = -3 e4,$   
 $[e4, e9] = 3 e6, [e5, e6] = -2 e1, [e5, e7] = e5, [e5, e8] = e6, [e5, e9] = -3 e3, [e6, e7] = -e6, [e6, e8] = e4, [e6, e9] = 4 e5, [e7, e8]$   
 $= 2 e8, [e7, e9] = -2 e9, [e8, e9] = e7]$

(148)

(149)

```
sym > DGsetup(LieAlgebraData([e1,evalDG(2*e2),e3,e4,e5,e6,e7,e8,e9],sym));
Lie algebra: sym
```

```
sym > gene1:=e3:gene2:=evalDG(add(c2||i*e||i,i=1..9)):gene3:=evalDG(add(c3||i*e||i,i=1..9)):
```

We need to find the most general embedding of  $l_1$  which admits a non-degenerate almost complex structure on the isotropy. We know from the solutions above that  $e_3$  from  $V^4$  can be included in this.

```
sym > eq1:=DGinfo(evalDG(LieBracket(gene2,gene3)+gene3),"CoefficientSet");
eq1 := {c32, 2 c27 c38 - 2 c28 c37 + c38, -2 c27 c39 + 2 c29 c37 + c39, c28 c39 - c29 c38 + c37, c22 c33 - c23 c32 + 3 c23 c37
```

(151)

```

- 3 c25 c39 - 3 c27 c33 + 3 c29 c35 + c33, c22 c34 - c24 c32 - 3 c24 c37 + c26 c38 + 3 c27 c34 - c28 c36 + c34, -2 c21 c32
+ 2 c22 c31 - 2 c23 c34 + 2 c24 c33 - 2 c25 c36 + 2 c26 c35 + c31, c22 c35 - c23 c38 - c25 c32 + c25 c37 + 4 c26 c39 - c27 c35
+ c28 c33 - 4 c29 c36 + c35, c22 c36 + 3 c24 c39 + c25 c38 - c26 c32 - c26 c37 + c27 c36 - c28 c35 - 3 c29 c34 + c36}
```

```
sym > eq2:=DGinfo(evalDG(LieBracket(gene3,gene1)),"CoefficientSet");
eq2 := {c38, 2 c34, -3 c37 + c32}
```

(152)

```
sym > eq3:=DGinfo(evalDG(LieBracket(gene2,gene1)+2*gene1),"CoefficientSet");
eq3 := {c28, 2 c24, 2 - 3 c27 + c22}
```

(153)

```
sym > vars:={seq(seq(c||i||j,j=1..9),i=1..3)};
vars := {c11, c12, c13, c14, c15, c16, c17, c18, c19, c21, c22, c23, c24, c25, c26, c27, c28, c29, c31, c32, c33, c34, c35, c36, c37, c38, c39}
```

(154)

```
sym > embedsols:=RealDomain[solve]({op(eq1),op(eq2),op(eq3)},vars):nops([%]);
4
```

(155)

Solve for the structure equations of  $l_1$ .

```
sym > DGsimplify(subs(embedsols[1],[gene2,gene3]));DGsimplify(subs(embedsols[2],[gene2,gene3]));
;DGsimplify(subs(embedsols[3],[gene2,gene3]));DGsimplify(subs(embedsols[4],[gene2,gene3]));
```

$$\left[ c_{21} e_1 - \left( \frac{5}{4} e_2 \right) + c_{23} e_3 + \frac{4 c_{26} c_{35} - 3 c_{31}}{4 c_{36}} e_5 + c_{26} e_6 + \frac{1}{4} e_7 - \left( \frac{c_{35}}{8 c_{36}} e_9 \right), c_{31} e_1 - \left( \frac{3 c_{35}^2}{8 c_{36}} e_3 \right) + c_{35} e_5 + c_{36} e_6 \right]$$

$$\left[ c_{21} e_1 - \left( \frac{1}{2} e_2 \right) + c_{23} e_3 + c_{25} e_5 + \frac{1}{2} e_7 + c_{29} e_9, c_{31} e_1 - ((3 c_{25} c_{39} - 3 c_{29} c_{35}) e_3) + c_{35} e_5 + c_{39} e_9 \right]$$

$$[c_{21} e_1 + (-2 + 3 c_{27}) e_2 + c_{23} e_3 + c_{25} e_5 + c_{26} e_6 + c_{27} e_7 + c_{29} e_9, 0 e_1]$$

$$\left[ c_{21} e_1 - \left( \frac{1}{2} e_2 \right) + c_{23} e_3 + c_{25} e_5 + c_{26} e_6 + \frac{1}{2} e_7 + c_{29} e_9, c_{31} e_1 \right]$$

(156)

Three out of four solution families are disregarded, because they contain too much intersection with the radical (again following our computations above).

```
sym > u1:=DGsimplify(subs(embedsols[2],gene2));u2:=DGsimplify(subs(embedsols[2],gene3));
```

$$u1 := c21 e1 - \left( \frac{1}{2} e2 \right) + c23 e3 + c25 e5 + \frac{1}{2} e7 + c29 e9$$

$$u2 := c31 e1 - ((3 c25 c39 - 3 c29 c35) e3) + c35 e5 + c39 e9 \quad (157)$$

```
sym > Iso:=[u1,u2,e3];
```

$$Iso := \left[ c21 e1 - \left( \frac{1}{2} e2 \right) + c23 e3 + c25 e5 + \frac{1}{2} e7 + c29 e9, c31 e1 - ((3 c25 c39 - 3 c29 c35) e3) + c35 e5 + c39 e9, e3 \right] \quad (158)$$

```
sym > adsym:=Adjoint(sym,representationSpace=sym):
```

```
sym > DGsetup(LieAlgebraData(Iso,iso)):
```

```
sym > resad:=RestrictedRepresentation(adsym,iso,Iso):
```

```
sym > ComplementaryBasis(Iso,DGinfo(sym,"FrameBaseVectors"));
[e1, e2, e4, e5, e6, e8] \quad (159)
```

```
sym > isocomp:=[e1,e2,e8,e4,e5,e6];
```

$$isocomp := [e1, e2, e8, e4, e5, e6] \quad (160)$$

```
sym > DGsetup([seq(r||i,i=1..6)],R6);
```

*frame name: R6* \quad (161)

```
sym > quotrep:=QuotientRepresentation(resad,Iso,isocomp,R6):
```

```
sym > mats:=DGinfo(quotrep,"RepresentationMatrices");
```

$$mats := \begin{bmatrix} -1 & -2 c21 & \frac{2 (c21 c39 - c29 c31) c29}{c39} & -2 c23 & 0 & -2 c25 \\ 0 & 0 & -c29 & 0 & 0 & 0 \\ 0 & 0 & 1 & 0 & 0 & 0 \\ 0 & 0 & 0 & 1 & 0 & 0 \\ 0 & -c25 & -c23 + \frac{2 (c25 c39 - c29 c35) c29}{c39} & 0 & -1 & -4 c29 \\ 0 & 0 & c25 & -3 c29 & 0 & 0 \end{bmatrix}, \quad (162)$$

$$\begin{bmatrix} 0 & -2 c_{31} & 2 c_{21} c_{39} - 2 c_{29} c_{31} & 6 c_{25} c_{39} - 6 c_{29} c_{35} & 0 & -2 c_{35} \\ 0 & 0 & -c_{39} & 0 & 0 & 0 \\ 0 & 0 & 0 & 0 & 0 & 0 \\ 0 & 0 & 0 & 0 & 0 & 0 \\ 0 & -c_{35} & 5 c_{25} c_{39} - 5 c_{29} c_{35} & 0 & 0 & -4 c_{39} \\ 0 & 0 & c_{35} & -3 c_{39} & 0 & 0 \end{bmatrix}, \begin{bmatrix} 0 & 0 & 0 & -2 & 0 & 0 \\ 0 & 0 & 0 & 0 & 0 & 0 \\ 0 & 0 & 0 & 0 & 0 & 0 \\ 0 & 0 & 0 & 0 & 0 & 0 \\ 0 & 0 & -1 & 0 & 0 & 0 \\ 0 & 0 & 0 & 0 & 0 & 0 \end{bmatrix}$$

```
sym > Endos:=GenerateTensors([DGinfo(R6,"FrameBaseVectors"),DGinfo(R6,"FrameBaseForms")]):
```

```
sym > invendos:=Invariants(quotrep,Endos);nops(%);
```

$$\begin{aligned} \text{invendos} := & \left[ D_{r1} dr1 + D_{r2} dr2 + D_{r3} dr3 + D_{r4} dr4 + D_{r5} dr5 + D_{r6} dr6, \left( \frac{c_{35}}{3 (c_{25} c_{39} - c_{29} c_{35})} D_{r1} \right) dr1 \right. \\ & + \left( \frac{c_{21} c_{35} - c_{25} c_{31}}{3 (c_{25} c_{39} - c_{29} c_{35})} D_{r1} \right) dr2 + \left( \frac{4 c_{39}^2 c_{21} - c_{35} c_{39} c_{25} - 4 c_{29} c_{31} c_{39} + c_{29} c_{35}^2}{6 c_{39}^2} D_{r1} \right) dr3 \\ & - \left( \left( \frac{c_{25} c_{39} - c_{29} c_{35}}{c_{39}} D_{r1} \right) dr4 \right) + \left( \frac{c_{31} c_{39} - c_{35}^2}{6 (c_{25} c_{39} - c_{29} c_{35}) c_{39}} D_{r1} \right) dr5 \\ & - \left( \left( \frac{2 (c_{39}^2 c_{21} - c_{35} c_{39} c_{25} - c_{29} c_{31} c_{39} + c_{29} c_{35}^2)}{3 (c_{25} c_{39} - c_{29} c_{35}) c_{39}} D_{r1} \right) dr6 \right) + \left( \frac{c_{35}}{6 (c_{25} c_{39} - c_{29} c_{35})} D_{r2} \right) dr2 - \left( \left( \frac{1}{3} D_{r2} \right) dr3 \right) \\ & + \left( \frac{c_{39}}{3 (c_{25} c_{39} - c_{29} c_{35})} D_{r2} \right) dr6 - \left( \left( \frac{c_{35}}{6 (c_{25} c_{39} - c_{29} c_{35})} D_{r3} \right) dr3 \right) + \left( \frac{c_{39}}{c_{25} c_{39} - c_{29} c_{35}} D_{r3} \right) dr4 \\ & + \left( \frac{c_{31} c_{39} - c_{35}^2}{12 (c_{25} c_{39} - c_{29} c_{35}) c_{39}} D_{r4} \right) dr3 + \left( \frac{c_{35}}{3 (c_{25} c_{39} - c_{29} c_{35})} D_{r4} \right) dr4 + \left( \frac{c_{39}}{2 (c_{25} c_{39} - c_{29} c_{35})} D_{r5} \right) dr1 \\ & + \left( \frac{3 c_{39}^2 c_{21} - c_{35} c_{39} c_{25} - 3 c_{29} c_{31} c_{39} + c_{29} c_{35}^2}{3 (c_{25} c_{39} - c_{29} c_{35}) c_{39}} D_{r5} \right) dr2 - \left( \left( \frac{c_{25} c_{39} - c_{29} c_{35}}{6 c_{39}} D_{r5} \right) dr3 \right) \\ & - \left( \left( \frac{c_{35}}{6 (c_{25} c_{39} - c_{29} c_{35})} D_{r5} \right) dr5 \right) + \left( \frac{2}{3} D_{r5} \right) dr6 + \left( \frac{3 c_{31} c_{39} - c_{35}^2}{12 (c_{25} c_{39} - c_{29} c_{35}) c_{39}} D_{r6} \right) dr2 - \left( \left( \frac{c_{35}}{6 c_{39}} D_{r6} \right) dr3 \right) \end{aligned}$$

$$+ D_{r6} dr4 \Big]$$

2

(163)

```
sym > jeqs:=DGinfo(evalDG(ContractIndices(invendos[2],invendos[2],[[2,1]])+1*invendos[1]),
  "CoefficientSet");
```

```
R6 > jsols:=solve(jeqs);
```

$$jsols := \{c21 = c21, c25 = c25, c29 = c29, c31 = -12 c25^2 c39 l, c35 = 0, c39 = c39, l = l\}$$

(164)

These equations give us those solutions which admit a structure J with  $J^2 = l \cdot Id$ , so almost complex, almost product or nilpotent.

```
sym > u1:=DGsimplify(subs(jsols,u1));u2:=DGsimplify(subs(jsols,u2));
```

$$u1 := c21 e1 - \left( \frac{1}{2} e2 \right) + c23 e3 + c25 e5 + \frac{1}{2} e7 + c29 e9$$

$$u2 := -(12 c25^2 c39 l e1) - (3 c25 c39 e3) + c39 e9$$

(165)

```
sym > multivec:=[<0,0,1,0,0,0,0,0,0>,subs(c23=0,subs(embedsols[2],<seq(c2||i,i=1..9)>)),<-12*
  c25^2*1,0,-3*c25,0,0,0,0,0,1>];
```

$$multivec := \left[ \begin{bmatrix} 0 \\ 0 \\ 1 \\ 0 \\ 0 \\ 0 \\ 0 \\ 0 \\ 0 \end{bmatrix}, \begin{bmatrix} c21 \\ -\frac{1}{2} \\ 0 \\ 0 \\ c25 \\ 0 \\ \frac{1}{2} \\ 0 \\ c29 \end{bmatrix}, \begin{bmatrix} -12 c25^2 l \\ 0 \\ -3 c25 \\ 0 \\ 0 \\ 0 \\ 0 \\ 0 \\ 1 \end{bmatrix} \right]$$

(166)

These vectors consist of the coefficients of the most general embedding. Now we apply inner automorphisms (conjugation) to reduce the number of parameters. This is done by exponentiating adjoint matrices.

```
sym > admats:=Adjoint();
```

```
sym > multivec:=subs({t=-c21},map(x->LinearAlgebra[MatrixExponential](admats[1],t).x,multivec))
```

;

$$multivec := \begin{bmatrix} \begin{bmatrix} 0 \\ 0 \\ 1 \\ 0 \\ 0 \\ 0 \\ 0 \\ 0 \\ 0 \end{bmatrix}, \begin{bmatrix} 0 \\ -\frac{1}{2} \\ 0 \\ 0 \\ c25 \\ 0 \\ \frac{1}{2} \\ 0 \\ c29 \end{bmatrix}, \begin{bmatrix} -12 \, c25^2 \, l \\ 0 \\ -3 \, c25 \\ 0 \\ 0 \\ 0 \\ 0 \\ 0 \\ 1 \end{bmatrix} \end{bmatrix} \quad (167)$$

```
sym > multivec:=subs({t=-c25},map(x->LinearAlgebra[MatrixExponential](admits[5],t).x,multivec))
;
```

$$multivec := \begin{bmatrix} \begin{bmatrix} 0 \\ 0 \\ 1 \\ 0 \\ 0 \\ 0 \\ 0 \\ 0 \\ 0 \end{bmatrix}, \begin{bmatrix} 0 \\ -\frac{1}{2} \\ 3 \, c29 \, c25 \\ 0 \\ 0 \\ 0 \\ 0 \\ \frac{1}{2} \\ 0 \\ c29 \end{bmatrix}, \begin{bmatrix} -12 \, c25^2 \, l \\ 0 \\ 0 \\ 0 \\ 0 \\ 0 \\ 0 \\ 0 \\ 1 \end{bmatrix} \end{bmatrix} \quad (168)$$

```
sym > multivec:=subs({t=-c29},map(x->LinearAlgebra[MatrixExponential](admits[9],t).x,multivec))
```

;

$$multivec := \begin{bmatrix} \begin{bmatrix} 0 \\ 0 \\ 1 \\ 0 \\ 0 \\ 0 \\ 0 \\ 0 \\ 0 \end{bmatrix}, \begin{bmatrix} 0 \\ -\frac{1}{2} \\ 3 c_{29} c_{25} \\ 0 \\ 0 \\ 0 \\ 0 \\ \frac{1}{2} \\ 0 \\ 0 \end{bmatrix}, \begin{bmatrix} -12 c_{25}^2 l \\ 0 \\ 0 \\ 0 \\ 0 \\ 0 \\ 0 \\ 0 \\ 1 \end{bmatrix} \end{bmatrix} \quad (169)$$

```
sym > multivec:=subs({t=-(3/2)*c25*c29},map(x->LinearAlgebra[MatrixExponential](admits[3],t).x,
multivec));
```

$$multivec := \begin{bmatrix} \begin{bmatrix} 0 \\ 0 \\ 1 \\ 0 \\ 0 \\ 0 \\ 0 \\ 0 \\ 0 \end{bmatrix}, \begin{bmatrix} 0 \\ -\frac{1}{2} \\ 0 \\ 0 \\ 0 \\ 0 \\ 0 \\ \frac{1}{2} \\ 0 \\ 0 \end{bmatrix}, \begin{bmatrix} -12 c_{25}^2 l \\ 0 \\ 0 \\ 0 \\ 0 \\ 0 \\ 0 \\ 0 \\ 1 \end{bmatrix} \end{bmatrix} \quad (170)$$

```
sym > subs({},map(x->LinearAlgebra[MatrixExponential](admits[2],t).x,multivec));
```

$$\left[ \begin{bmatrix} 0 \\ 0 \\ e^t \\ 0 \\ 0 \\ 0 \\ 0 \\ 0 \\ 0 \end{bmatrix}, \begin{bmatrix} 0 \\ -\frac{1}{2} \\ 0 \\ 0 \\ 0 \\ 0 \\ \frac{1}{2} \\ 0 \\ 0 \end{bmatrix}, \begin{bmatrix} -12 e^{2t} c 25^2 l \\ 0 \\ 0 \\ 0 \\ 0 \\ 0 \\ 0 \\ 0 \\ 1 \end{bmatrix} \right] \quad (171)$$

In the end, we see that there is only one discrete parameter left,  $l$ . This parameter determines the type of invariant structure. We may normalize it to  $l = -1$ , to get an almost complex structure. Thus the conjugacy class of  $l_1$  is unique. Now we need to verify that this structure is actually non-degenerate.

```
sym > ChangeFrame(sym);
```

*sym* (172)

```
sym > Iso:=[evalDG(-(1/2)*e2+(1/2)*e7),evalDG(1*e1+e9),e3];
```

$$Iso := \left[ -\left( \frac{1}{2} e2 \right) + \frac{1}{2} e7, l e1 + e9, e3 \right] \quad (173)$$

```
sym > DGsetup(LieAlgebraData(Iso,iso)):
```

```
sym > resad:=RestrictedRepresentation(adsym,iso,Iso):
```

```
sym > ComplementaryBasis(Iso,DGinfo(sym,"FrameBaseVectors"));
```

*[e1, e2, e4, e5, e6, e8]* (174)

```
sym > isocomp:=[e1,e2,e8,e4,e5,e6];
```

*isocomp := [e1, e2, e8, e4, e5, e6]* (175)

```
sym > DGsetup([seq(r||i,i=1..6)],R6);
```

*frame name: R6* (176)

```
sym > quotrep:=QuotientRepresentation(resad,Iso,isocomp,R6):
```

```
sym > mats:=DGinfo(quotrep,"RepresentationMatrices");
```



$$mats := \left[ \begin{bmatrix} -1 & 0 & 0 & 0 & 0 & 0 \\ 0 & 0 & 0 & 0 & 0 & 0 \\ 0 & 0 & 1 & 0 & 0 & 0 \\ 0 & 0 & 0 & 1 & 0 & 0 \\ 0 & 0 & 0 & 0 & -1 & 0 \\ 0 & 0 & 0 & 0 & 0 & 0 \end{bmatrix}, \begin{bmatrix} 0 & -2l & 0 & 0 & 0 & 0 \\ 0 & 0 & -1 & 0 & 0 & 0 \\ 0 & 0 & 0 & 0 & 0 & 0 \\ 0 & 0 & 0 & 0 & 0 & 0 \\ 0 & 0 & 0 & 0 & 0 & -4 \\ 0 & 0 & 0 & -3 & 0 & 0 \end{bmatrix}, \begin{bmatrix} 0 & 0 & 0 & -2 & 0 & 0 \\ 0 & 0 & 0 & 0 & 0 & 0 \\ 0 & 0 & 0 & 0 & 0 & 0 \\ 0 & 0 & 0 & 0 & 0 & 0 \\ 0 & 0 & -1 & 0 & 0 & 0 \\ 0 & 0 & 0 & 0 & 0 & 0 \end{bmatrix} \right] \quad (177)$$

```
sym > Endos:=GenerateTensors([DGinfo(R6,"FrameBaseVectors"),DGinfo(R6,"FrameBaseForms")]):
sym > invendos:=Invariants(quotrep,Endos);nops(%);
```

$$invendos := \left[ D_{r1} dr1 + D_{r2} dr2 + D_{r3} dr3 + D_{r4} dr4 + D_{r5} dr5 + D_{r6} dr6, \left( \frac{2}{3} D_{r1} \right) dr5 + \left( \frac{4}{3l} D_{r2} \right) dr6 + \left( \frac{4}{l} D_{r3} \right) dr4 \right. \\ \left. + \left( \frac{1}{3} D_{r4} \right) dr3 + \left( \frac{2}{l} D_{r5} \right) dr1 + D_{r6} dr2 \right]$$

2

```
sym > DGinfo(evalDG(ContractIndices(invendos[2],invendos[2],[[2,1]])), "CoefficientSet");
```

$$\left\{ \frac{4}{3l} \right\}$$

```
sym > Jtencomps:=GetComponents(invendos[2],Endos);
```

$$Jtencomps := \left[ 0, 0, 0, 0, \frac{2}{3}, 0, 0, 0, 0, 0, 0, \frac{4}{3l}, 0, 0, 0, \frac{4}{l}, 0, 0, 0, 0, \frac{1}{3}, 0, 0, 0, \frac{2}{l}, 0, 0, 0, 0, 0, 0, 1, 0, 0, 0, 0 \right]$$

Get the components of the invariant structure on the isotropy representation.

```
sym > ChangeFrame(sym);
```

R6

```
sym > compbas:=[e1,e2,e8,e4,e5,e6];
```

$$compbas := [e1, e2, e8, e4, e5, e6]$$

```
sym > compforms:=Annihilator(Iso);
```

$$compforms := \left[ -\left( \frac{1}{l} \theta 1 \right) + \theta 9, \theta 8, \theta 2 + \theta 7, \theta 6, \theta 5, \theta 4 \right]$$

```
sym > compforms:=[op(compforms[1..2]),compforms[6],op(compforms[3..5])];
```

$$compforms := \left[ -\left( \frac{1}{l} \theta 1 \right) + \theta 9, \theta 8, \theta 4, \theta 2 + \theta 7, \theta 6, \theta 5 \right]$$

```
sym > gendos:=GenerateTensors([compbas,compforms]);
```

$$\begin{aligned} \text{gendos} := & \left[ - \left( \left( \frac{1}{l} e1 \right) \theta1 \right) + e1 \theta9, e1 \theta8, e1 \theta4, e1 \theta2 + e1 \theta7, e1 \theta6, e1 \theta5, - \left( \left( \frac{1}{l} e2 \right) \theta1 \right) + e2 \theta9, e2 \theta8, e2 \theta4, e2 \theta2 + e2 \theta7, e2 \theta6, \right. \\ & e2 \theta5, - \left( \left( \frac{1}{l} e8 \right) \theta1 \right) + e8 \theta9, e8 \theta8, e8 \theta4, e8 \theta2 + e8 \theta7, e8 \theta6, e8 \theta5, - \left( \left( \frac{1}{l} e4 \right) \theta1 \right) + e4 \theta9, e4 \theta8, e4 \theta4, e4 \theta2 + e4 \theta7, e4 \theta6, \\ & e4 \theta5, - \left( \left( \frac{1}{l} e5 \right) \theta1 \right) + e5 \theta9, e5 \theta8, e5 \theta4, e5 \theta2 + e5 \theta7, e5 \theta6, e5 \theta5, - \left( \left( \frac{1}{l} e6 \right) \theta1 \right) + e6 \theta9, e6 \theta8, e6 \theta4, e6 \theta2 + e6 \theta7, e6 \theta6, \\ & \left. e6 \theta5 \right] \end{aligned} \quad (185)$$

```
sym > Jten:=evalDG(add(Jtencomps[i]*gendos[i],i=1..nops(gendos)));
```

$$Jten := \left( \frac{2}{3} e1 \right) \theta6 + \left( \frac{4}{3l} e2 \right) \theta5 + \left( \frac{1}{3} e4 \right) \theta4 - \left( \left( \frac{2}{l^2} e5 \right) \theta1 \right) + \left( \frac{2}{l} e5 \right) \theta9 + e6 \theta8 + \left( \frac{4}{l} e8 \right) \theta2 + \left( \frac{4}{l} e8 \right) \theta7 \quad (186)$$

Now we use the components from earlier to obtain a tensor on g which projects to the isotropy invariant almost complex structure.

```
sym > NJ:=TensorBrackets(Jten,Jten,"Frolicher-Nijenhuis");
```

$$\begin{aligned} NJ := & -\frac{64}{3l} e1 \otimes \theta1 \otimes \theta2 - \frac{128}{3l} e1 \otimes \theta1 \otimes \theta7 + \frac{64}{3l} e1 \otimes \theta2 \otimes \theta1 - \frac{64}{3} e1 \otimes \theta2 \otimes \theta9 - \frac{256}{9l} e1 \otimes \theta5 \otimes \theta6 + \frac{256}{9l} e1 \otimes \theta6 \otimes \theta5 \\ & + \frac{128}{3l} e1 \otimes \theta7 \otimes \theta1 - \frac{128}{3} e1 \otimes \theta7 \otimes \theta9 + \frac{64}{3} e1 \otimes \theta9 \otimes \theta2 + \frac{128}{3} e1 \otimes \theta9 \otimes \theta7 - \frac{128}{3l^2} e2 \otimes \theta1 \otimes \theta8 + \frac{256}{3l^2} e2 \otimes \theta4 \otimes \theta5 \\ & - \frac{256}{3l^2} e2 \otimes \theta5 \otimes \theta4 + \frac{128}{3l^2} e2 \otimes \theta8 \otimes \theta1 - \frac{128}{3l} e2 \otimes \theta8 \otimes \theta9 + \frac{128}{3l} e2 \otimes \theta9 \otimes \theta8 + \frac{64}{3l} e4 \otimes \theta2 \otimes \theta4 - \frac{64}{3l} e4 \otimes \theta4 \otimes \theta2 \\ & - \frac{128}{3l} e4 \otimes \theta4 \otimes \theta7 + \frac{128}{9l} e4 \otimes \theta6 \otimes \theta8 + \frac{128}{3l} e4 \otimes \theta7 \otimes \theta4 - \frac{128}{9l} e4 \otimes \theta8 \otimes \theta6 + \frac{256}{3l^2} e5 \otimes \theta1 \otimes \theta6 - \frac{64}{3l} e5 \otimes \theta2 \otimes \theta5 \\ & + \frac{64}{3l} e5 \otimes \theta5 \otimes \theta2 + \frac{128}{3l} e5 \otimes \theta5 \otimes \theta7 - \frac{256}{3l^2} e5 \otimes \theta6 \otimes \theta1 + \frac{256}{3l} e5 \otimes \theta6 \otimes \theta9 - \frac{128}{3l} e5 \otimes \theta7 \otimes \theta5 - \frac{256}{3l} e5 \otimes \theta9 \otimes \theta6 \\ & + \frac{64}{l^2} e6 \otimes \theta1 \otimes \theta4 - \frac{64}{l^2} e6 \otimes \theta4 \otimes \theta1 + \frac{64}{l} e6 \otimes \theta4 \otimes \theta9 + \frac{32}{3l} e6 \otimes \theta5 \otimes \theta8 - \frac{32}{3l} e6 \otimes \theta8 \otimes \theta5 - \frac{64}{l} e6 \otimes \theta9 \otimes \theta4 - \frac{64}{3l} e8 \\ & \otimes \theta2 \otimes \theta8 + \frac{512}{3l^2} e8 \otimes \theta4 \otimes \theta6 - \frac{512}{3l^2} e8 \otimes \theta6 \otimes \theta4 - \frac{128}{3l} e8 \otimes \theta7 \otimes \theta8 + \frac{64}{3l} e8 \otimes \theta8 \otimes \theta2 + \frac{128}{3l} e8 \otimes \theta8 \otimes \theta7 \end{aligned} \quad (187)$$

```
sym > comp_proj:=evalDG(add(compforms[i] &t compbas[i],i=1..6));
```

$$\text{comp\_proj} := \theta1 \otimes e1 + \theta2 \otimes e2 + \theta4 \otimes e4 + \theta5 \otimes e5 + \theta6 \otimes e6 + 2 \theta7 \otimes e2 + \theta8 \otimes e8 - l \theta9 \otimes e1 \quad (188)$$

```
sym > seq(ContractIndices(evalDG(comp_proj &t comp_proj),LieDerivative(Iso[i],Jten),[[1,1],[4,2]]),i=1..3);
```

$$0 e1 \otimes \theta1, 0 e1 \otimes \theta1, 0 e1 \otimes \theta1 \quad (189)$$

We verify that the structure Jten is in fact invariant modulo the isotropy subalgebra.

```
sym > ContractIndices(comp_proj &t comp_proj &t comp_proj, NJ, [[1,1],[4,2],[6,3]]);
```

$$\begin{aligned} & -\frac{64}{3l} e1 \otimes \theta1 \otimes \theta2 - \frac{128}{3l} e1 \otimes \theta1 \otimes \theta7 + \frac{64}{3l} e1 \otimes \theta2 \otimes \theta1 - \frac{64}{3} e1 \otimes \theta2 \otimes \theta9 - \frac{256}{9l} e1 \otimes \theta5 \otimes \theta6 + \frac{256}{9l} e1 \otimes \theta6 \otimes \theta5 + \frac{128}{3l} e1 \\ & \otimes \theta7 \otimes \theta1 - \frac{128}{3} e1 \otimes \theta7 \otimes \theta9 + \frac{64}{3} e1 \otimes \theta9 \otimes \theta2 + \frac{128}{3} e1 \otimes \theta9 \otimes \theta7 - \frac{128}{3l^2} e2 \otimes \theta1 \otimes \theta8 + \frac{256}{3l^2} e2 \otimes \theta4 \otimes \theta5 - \frac{256}{3l^2} e2 \otimes \theta5 \\ & \otimes \theta4 + \frac{128}{3l^2} e2 \otimes \theta8 \otimes \theta1 - \frac{128}{3l} e2 \otimes \theta8 \otimes \theta9 + \frac{128}{3l} e2 \otimes \theta9 \otimes \theta8 + \frac{64}{3l} e4 \otimes \theta2 \otimes \theta4 - \frac{64}{3l} e4 \otimes \theta4 \otimes \theta2 - \frac{128}{3l} e4 \otimes \theta4 \otimes \theta7 \\ & + \frac{128}{9l} e4 \otimes \theta6 \otimes \theta8 + \frac{128}{3l} e4 \otimes \theta7 \otimes \theta4 - \frac{128}{9l} e4 \otimes \theta8 \otimes \theta6 + \frac{256}{3l^2} e5 \otimes \theta1 \otimes \theta6 - \frac{64}{3l} e5 \otimes \theta2 \otimes \theta5 + \frac{64}{3l} e5 \otimes \theta5 \otimes \theta2 \\ & + \frac{128}{3l} e5 \otimes \theta5 \otimes \theta7 - \frac{256}{3l^2} e5 \otimes \theta6 \otimes \theta1 + \frac{256}{3l} e5 \otimes \theta6 \otimes \theta9 - \frac{128}{3l} e5 \otimes \theta7 \otimes \theta5 - \frac{256}{3l} e5 \otimes \theta9 \otimes \theta6 + \frac{64}{l^2} e6 \otimes \theta1 \otimes \theta4 \\ & - \frac{64}{l^2} e6 \otimes \theta4 \otimes \theta1 + \frac{64}{l} e6 \otimes \theta4 \otimes \theta9 + \frac{32}{3l} e6 \otimes \theta5 \otimes \theta8 - \frac{32}{3l} e6 \otimes \theta8 \otimes \theta5 - \frac{64}{l} e6 \otimes \theta9 \otimes \theta4 - \frac{64}{3l} e8 \otimes \theta2 \otimes \theta8 + \frac{512}{3l^2} e8 \\ & \otimes \theta4 \otimes \theta6 - \frac{512}{3l^2} e8 \otimes \theta6 \otimes \theta4 - \frac{128}{3l} e8 \otimes \theta7 \otimes \theta8 + \frac{64}{3l} e8 \otimes \theta8 \otimes \theta2 + \frac{128}{3l} e8 \otimes \theta8 \otimes \theta7 \end{aligned} \quad (190)$$

The projection of the Nijenhuis tensor on G gives the Nijenhuis tensor on m. We can see that it is non-degenerate, because its image is surjective.
